# Supplementary material for: Blink: Fast and Generic Collectives for Distributed ML
Source: arXiv:1910.04940 source file (2019-10-11)
Supplement: Supplementary file 1 [file appendix.tex]

\clearpage
\newpage

\section*{APPENDIX}

%\clearpage
%\newpage
\subsection{DGX-1-V100}

\begin{figure*}[h]
\centering
\subfigure[Fan-in forward throughput]{\label{fig:awsP3-1-fan-in-f}
\includegraphics[width=0.32\textwidth]{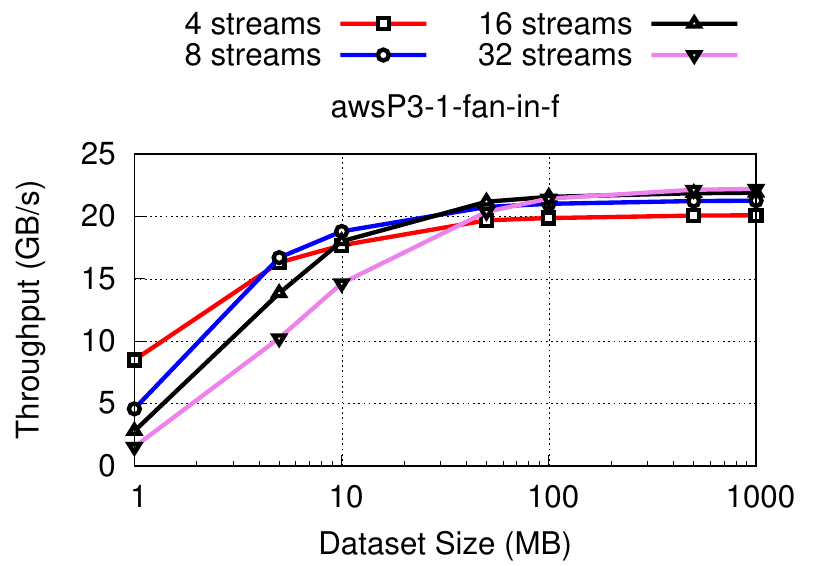}}
\subfigure[Fan-in reduce+forward throughput]{\label{fig:awsP3-1-fan-in-af} 
\includegraphics[width=0.32\textwidth]{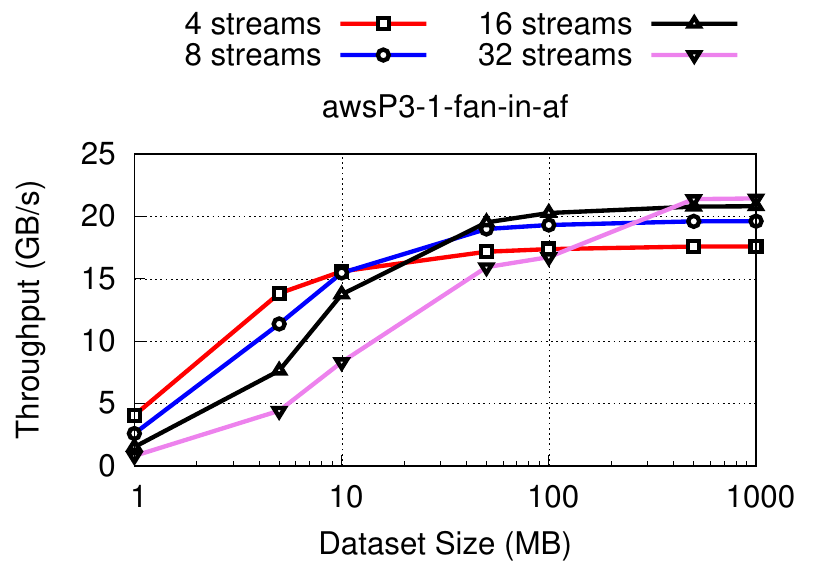}}
\subfigure[Fan-out forward throughput]{\label{fig:awsP3-1-fan-out-f} 
\includegraphics[width=0.32\textwidth]{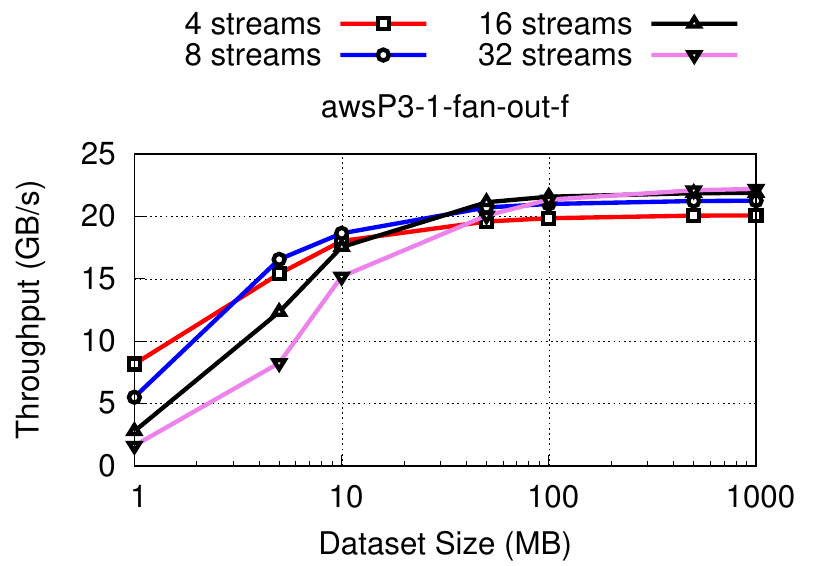}}
\subfigure[Fan-in forward throughput]{\label{fig:awsP3-2-fan-in-f}
\includegraphics[width=0.32\textwidth]{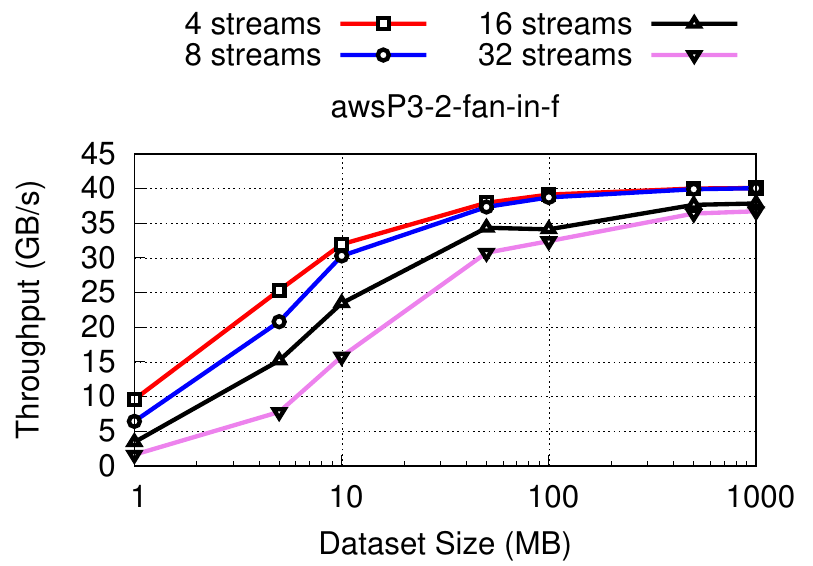}}
\subfigure[Fan-in reduce+forward throughput]{\label{fig:awsP3-2-fan-in-af} 
\includegraphics[width=0.32\textwidth]{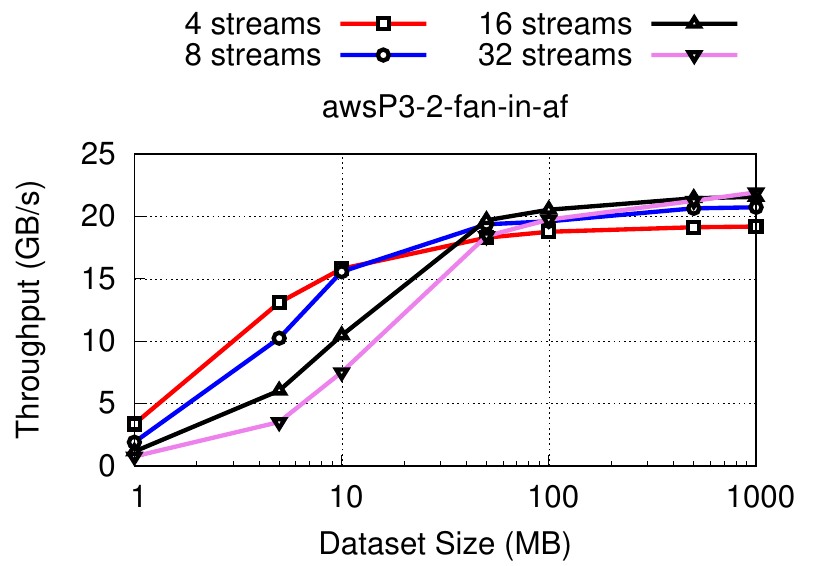}}
\subfigure[Fan-out forward throughput]{\label{fig:awsP3-2-fan-out-f} 
\includegraphics[width=0.32\textwidth]{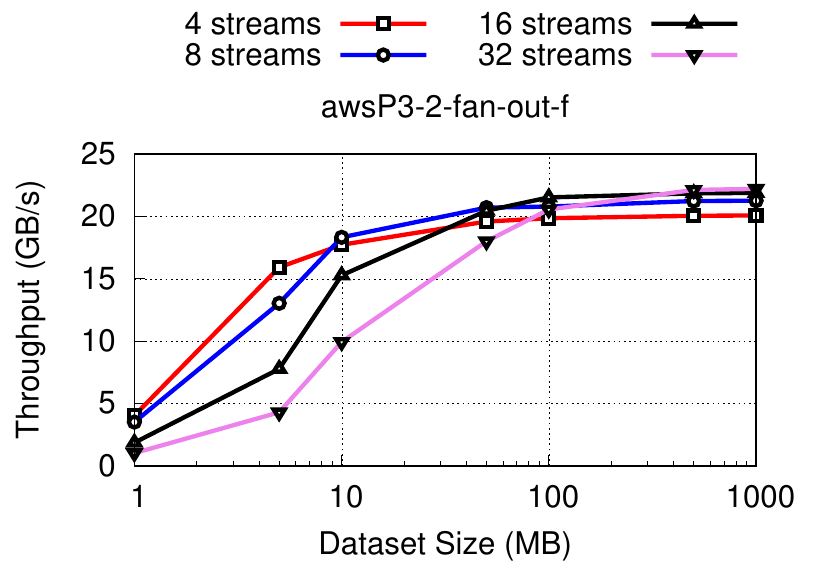}}
\subfigure[Fan-in forward throughput]{\label{fig:awsP3-3-fan-in-f}
\includegraphics[width=0.32\textwidth]{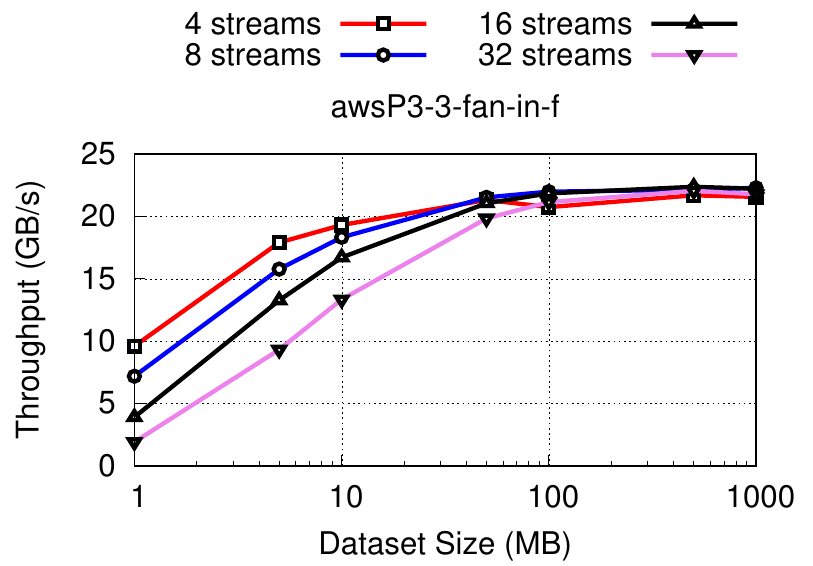}}
\subfigure[Fan-in reduce+forward throughput]{\label{fig:awsP3-3-fan-in-af} 
\includegraphics[width=0.32\textwidth]{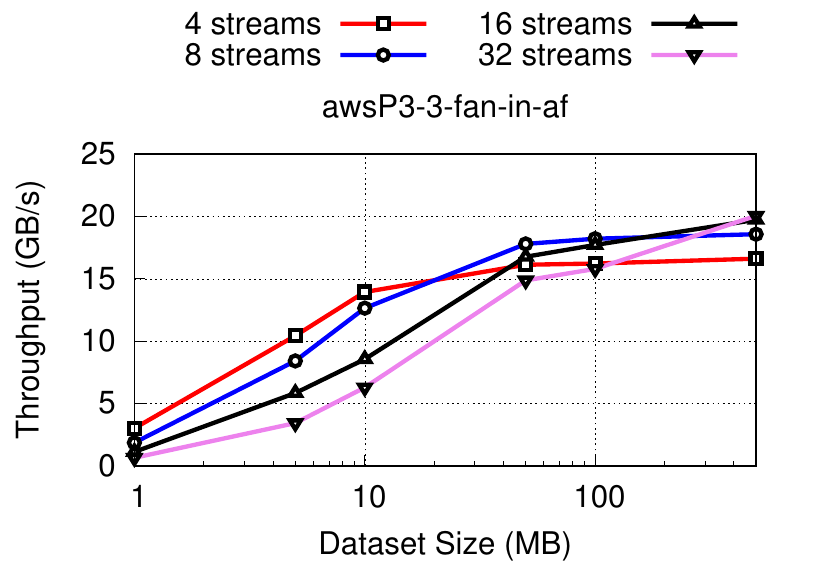}}
\subfigure[Fan-out forward throughput]{\label{fig:awsP3-3-fan-out-f} 
\includegraphics[width=0.32\textwidth]{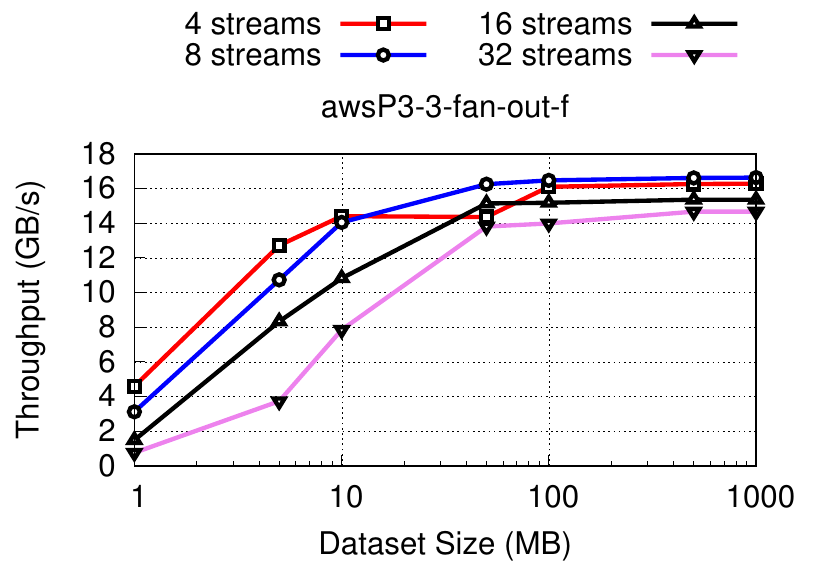}}
\vspace{-3mm}
\label{fig:aws-fanin-fanout}
\caption{AWS Fan-in forward, add+forward, Fan-out forward}
\vspace{-3mm}
\end{figure*}

\begin{figure*}[h]
\centering
\subfigure[MIMO]{\label{fig:awsP3-2i2o-af}
\includegraphics[width=0.32\textwidth]{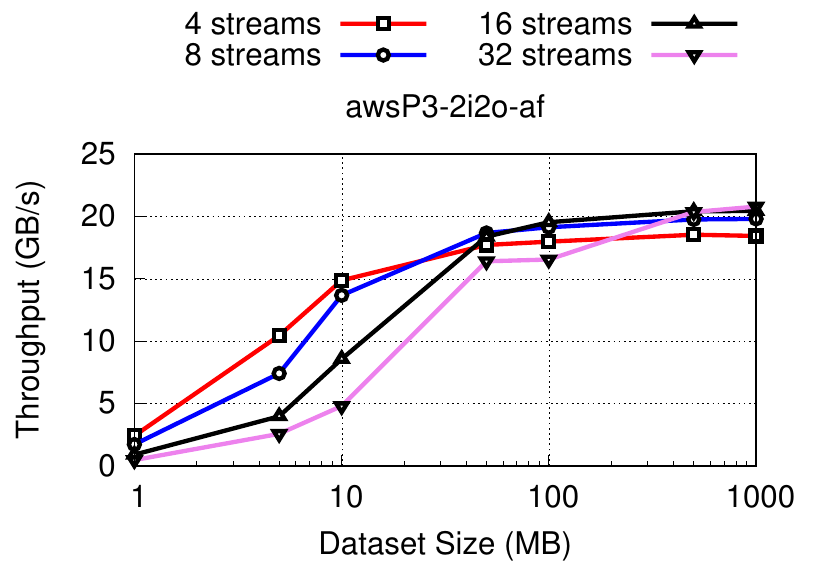}}
\subfigure[MCA]{\label{fig:awsP3-mc-af} 
\includegraphics[width=0.32\textwidth]{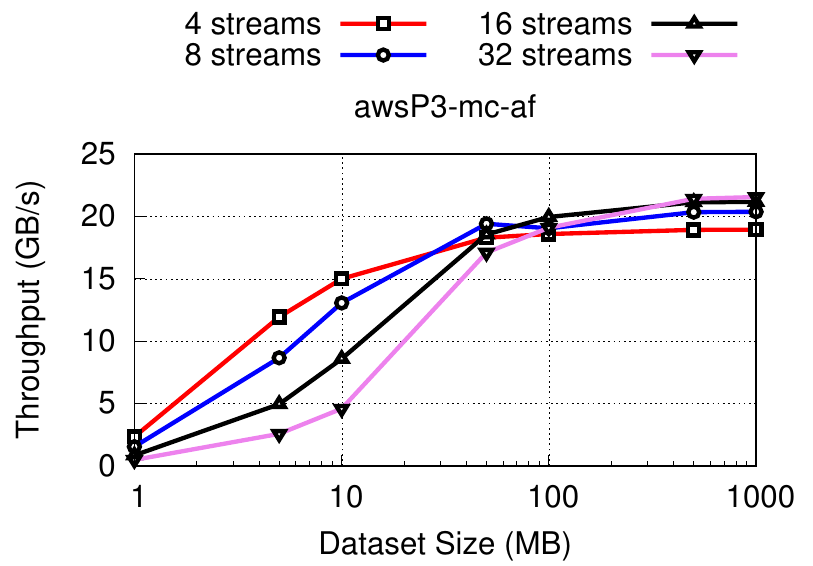}}
\vspace{-3mm}
\label{fig:aws-mimo-mca}
\caption{AWS MIMO MCA}
\vspace{-3mm}
\end{figure*}

\begin{figure*}[h]
\centering
\subfigure[3 GPU chain forward]{\label{fig:awsP3-3-chain-f}
\includegraphics[width=0.32\textwidth]{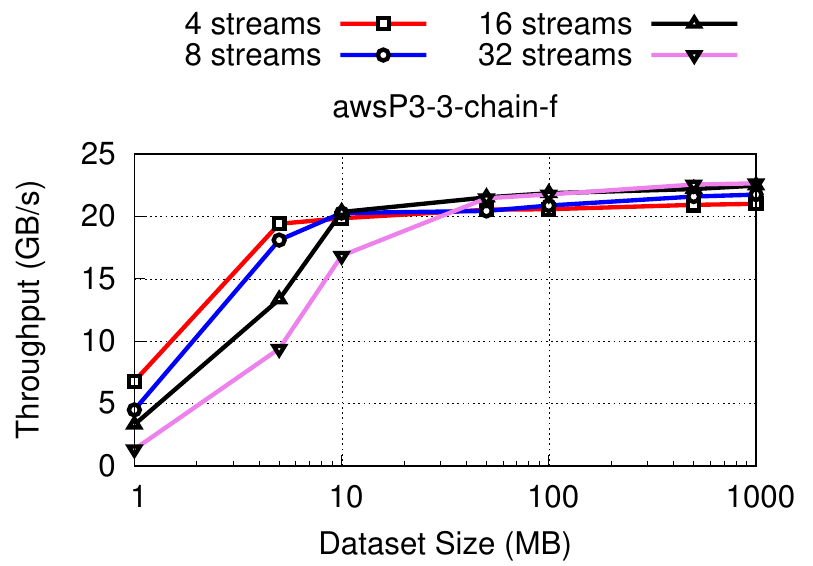}}
\subfigure[3 GPU chain reduce+forward]{\label{fig:awsP3-3-chain-af} 
\includegraphics[width=0.32\textwidth]{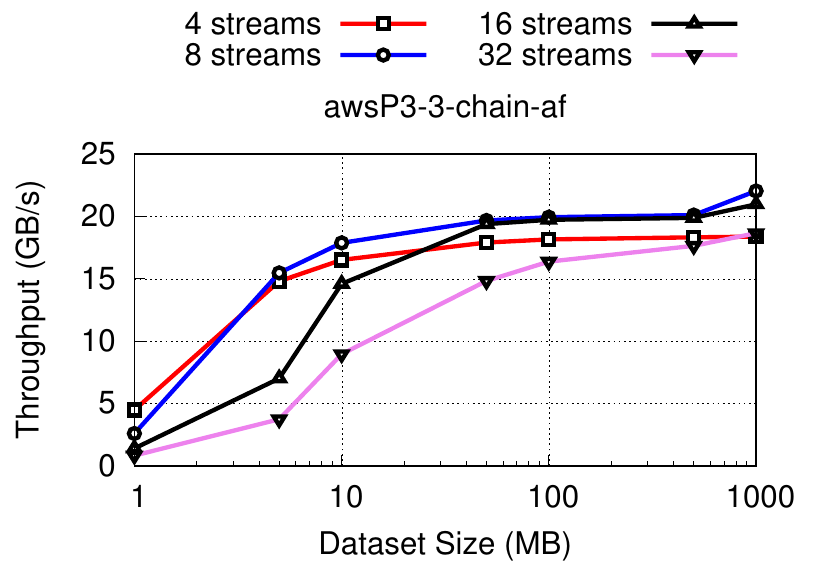}}
\subfigure[3 GPU chain reduce+bcast]{\label{fig:awsP3-3-reduce-bcast} 
\includegraphics[width=0.32\textwidth]{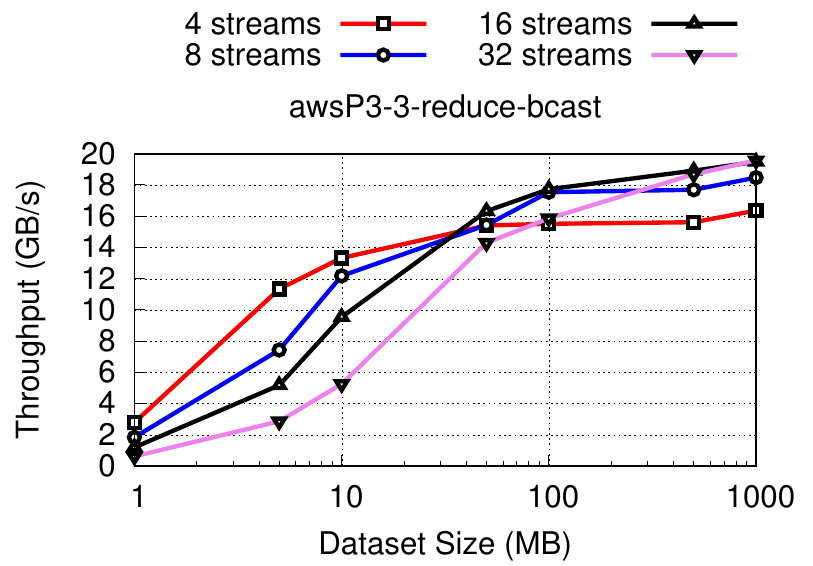}}
\subfigure[4 GPU chain forward]{\label{fig:awsP3-4-chain-f}
\includegraphics[width=0.32\textwidth]{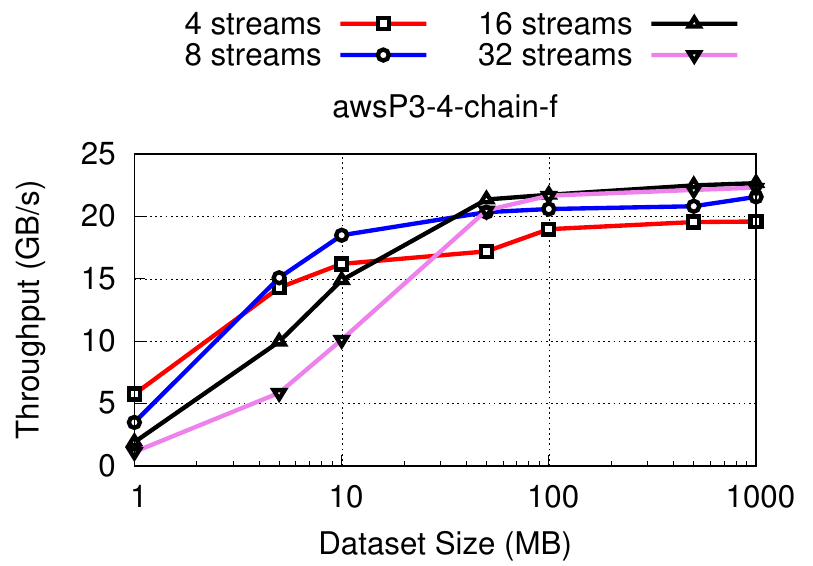}}
\subfigure[4 GPU chain reduce+forward]{\label{fig:awsP3-4-chain-af} 
\includegraphics[width=0.32\textwidth]{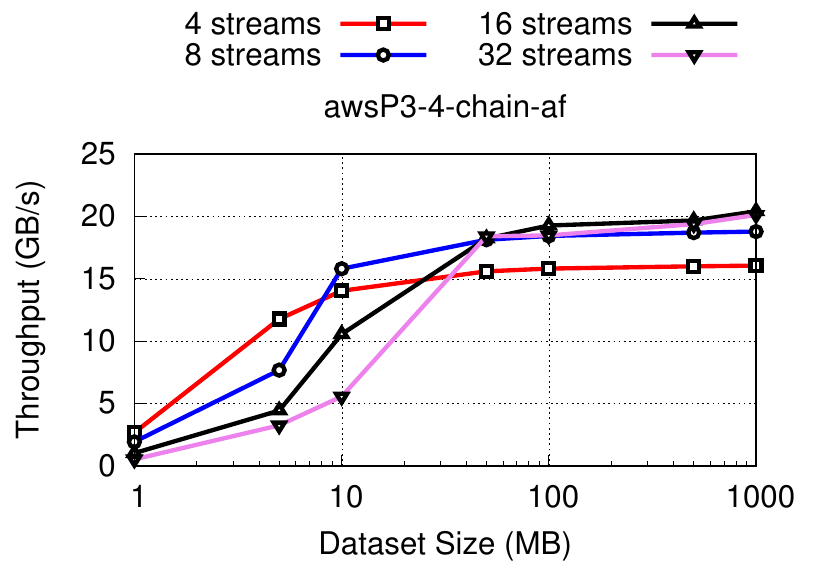}}
\subfigure[4 GPU chain reduce+bcast]{\label{fig:awsP3-4-reduce-bcast} 
\includegraphics[width=0.32\textwidth]{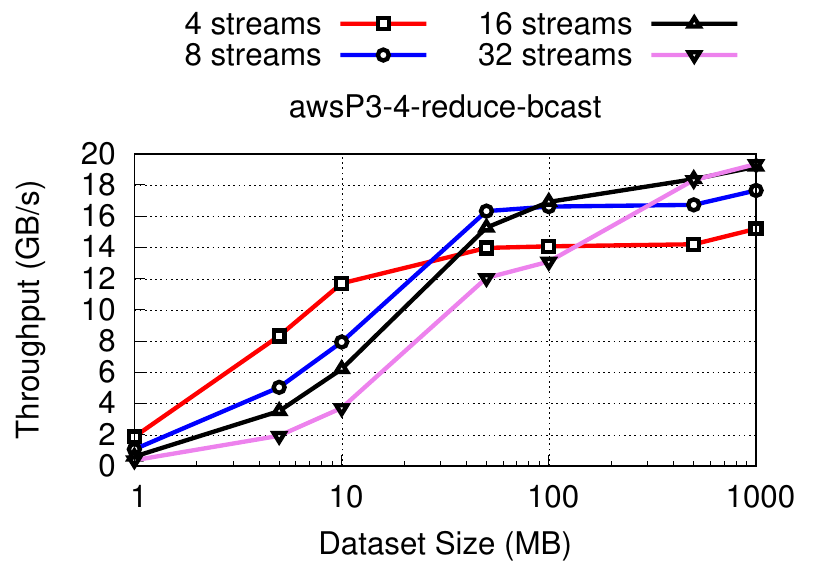}}
\subfigure[5 GPU chain forward]{\label{fig:awsP3-5-chain-f}
\includegraphics[width=0.32\textwidth]{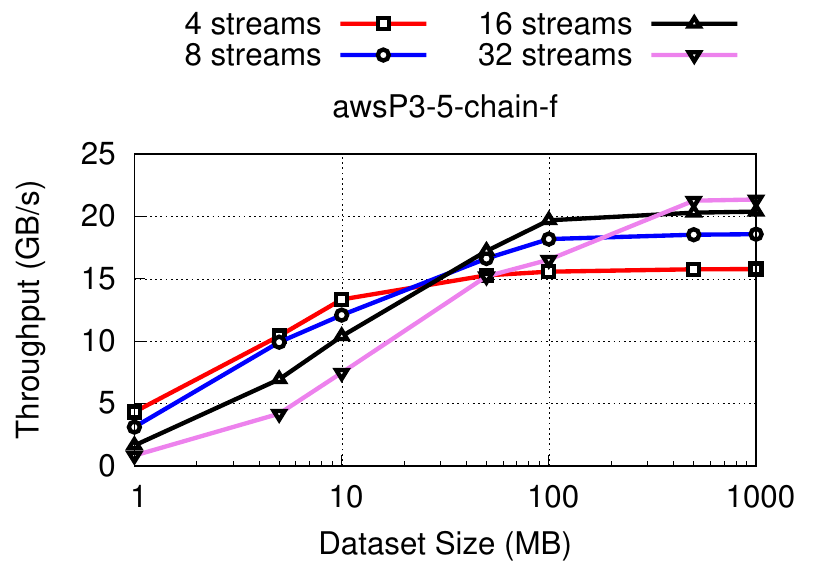}}
\subfigure[5 GPU chain reduce+forward]{\label{fig:awsP3-5-chain-af} 
\includegraphics[width=0.32\textwidth]{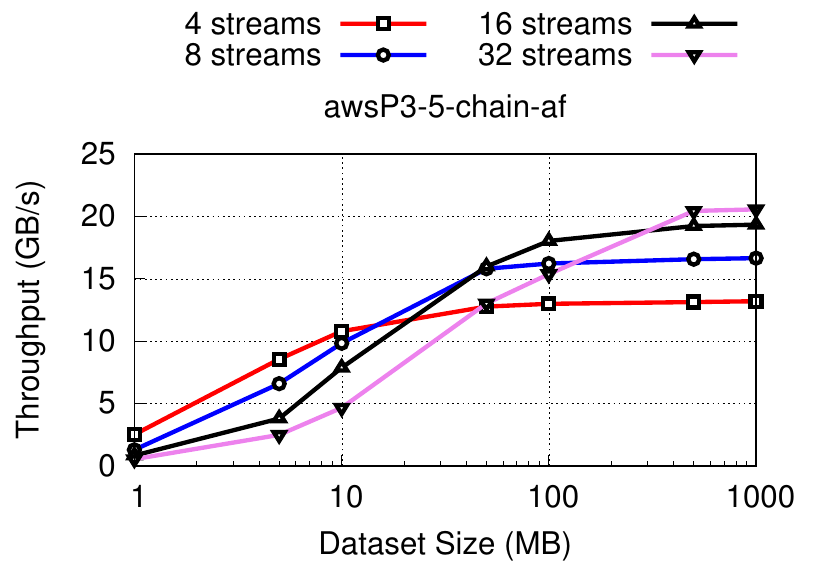}}
\subfigure[5 GPU chain reduce+bcast]{\label{fig:awsP3-5-reduce-bcast} 
\includegraphics[width=0.32\textwidth]{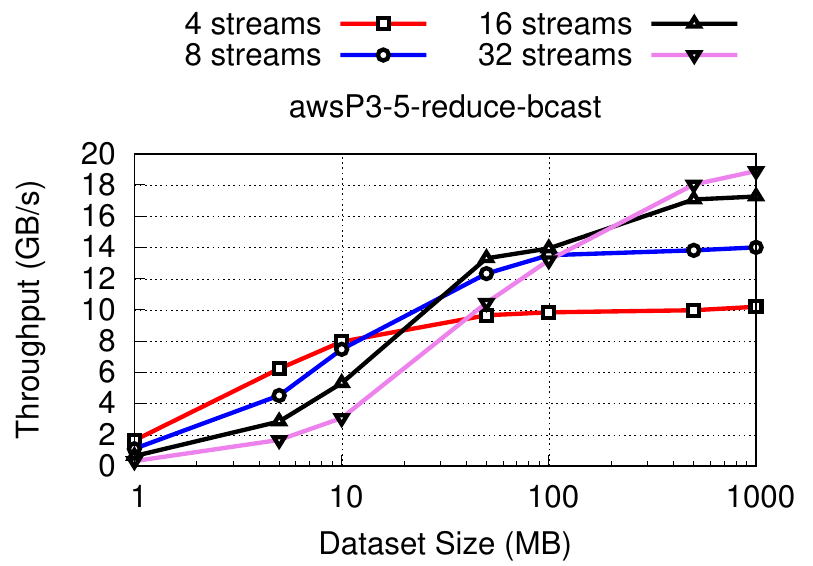}}
\vspace{-3mm}
\label{fig:aws-345-chain}
\caption{AWS 3,4,5 chain forward, reduce+forward, reduce-bcast}
\vspace{-3mm}
\end{figure*}

\begin{figure*}[h]
\centering
\subfigure[6 GPU chain forward]{\label{fig:awsP3-6-chain-f}
\includegraphics[width=0.32\textwidth]{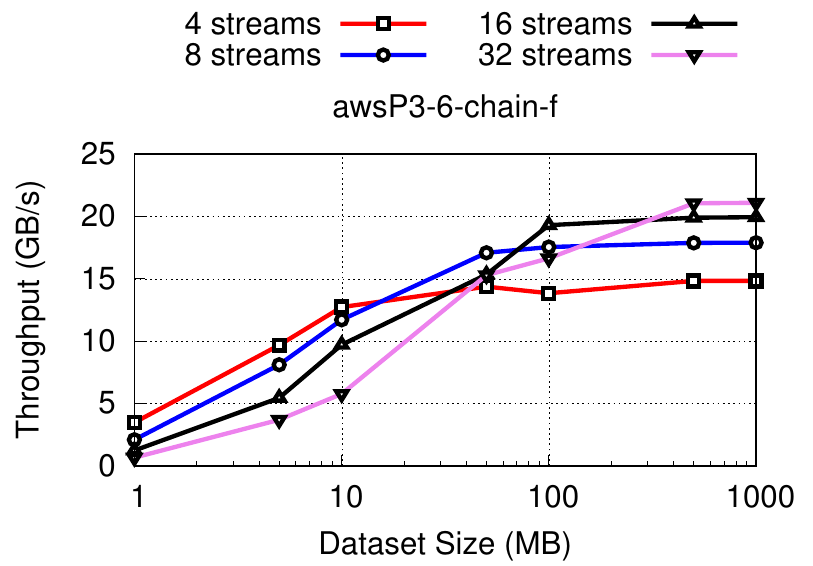}}
\subfigure[6 GPU chain reduce+forward]{\label{fig:awsP3-6-chain-af} 
\includegraphics[width=0.32\textwidth]{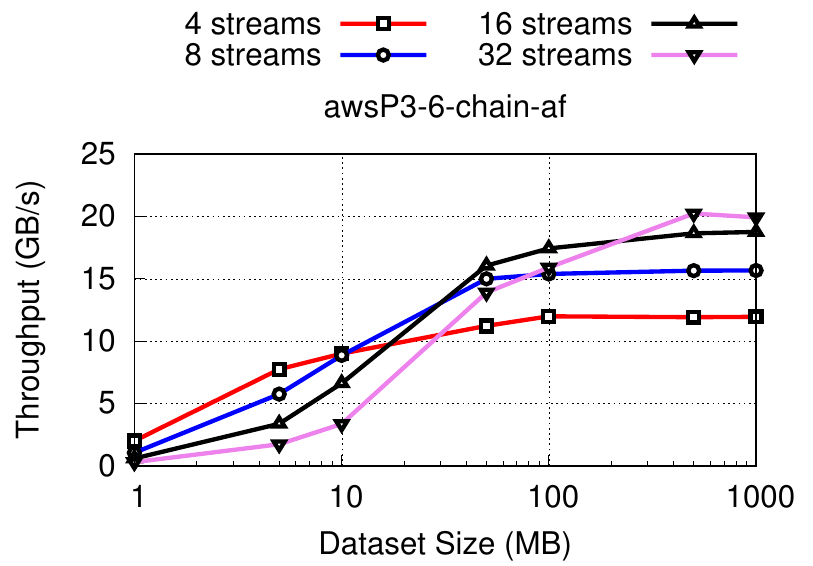}}
\subfigure[6 GPU chain reduce+bcast]{\label{fig:awsP3-6-reduce-bcast} 
\includegraphics[width=0.32\textwidth]{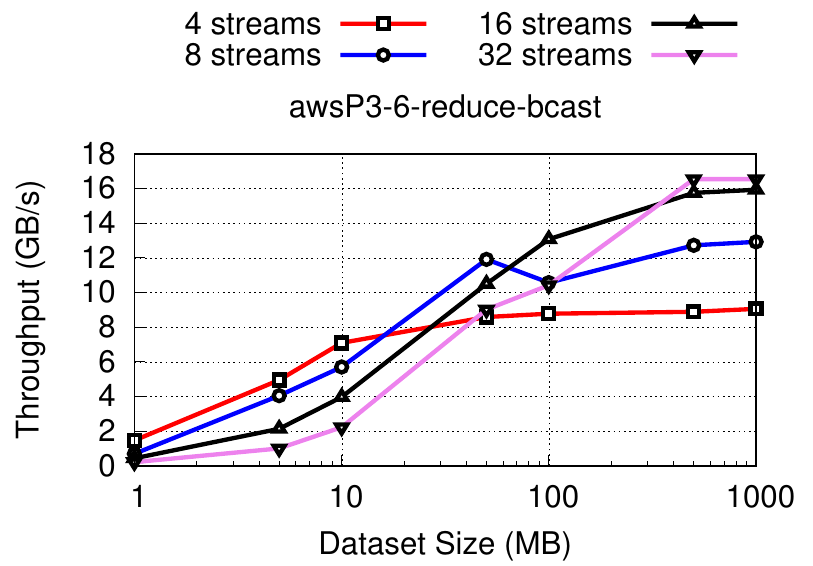}}
\subfigure[7 GPU chain forward]{\label{fig:awsP3-7-chain-f}
\includegraphics[width=0.32\textwidth]{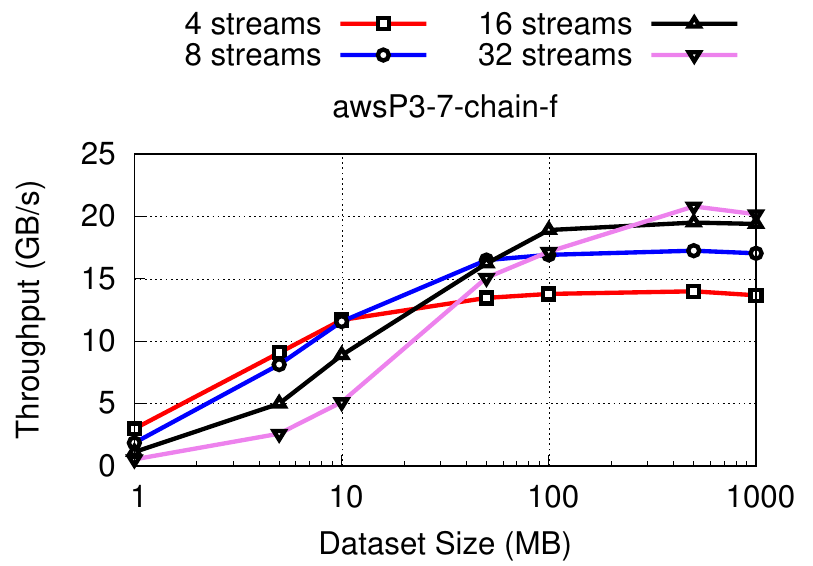}}
\subfigure[7 GPU chain reduce+forward]{\label{fig:awsP3-7-chain-af} 
\includegraphics[width=0.32\textwidth]{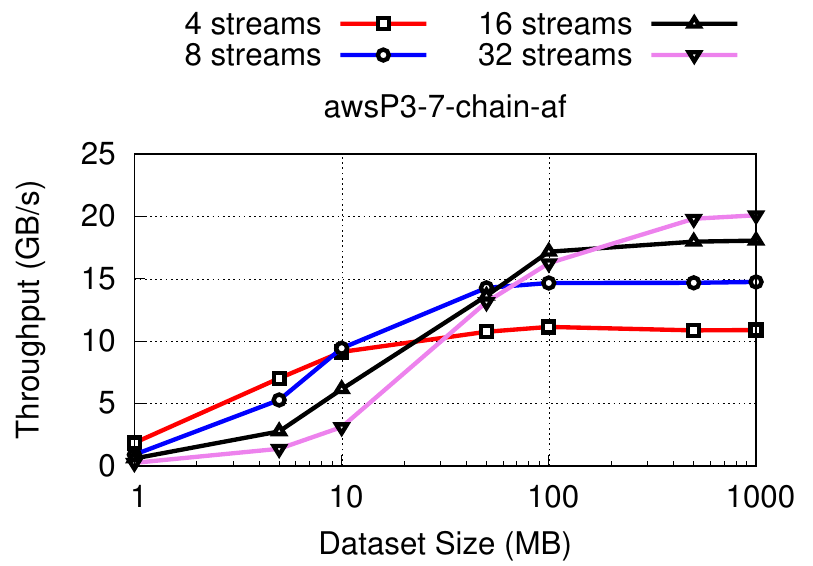}}
\subfigure[7 GPU chain reduce+bcast]{\label{fig:awsP3-7-reduce-bcast} 
\includegraphics[width=0.32\textwidth]{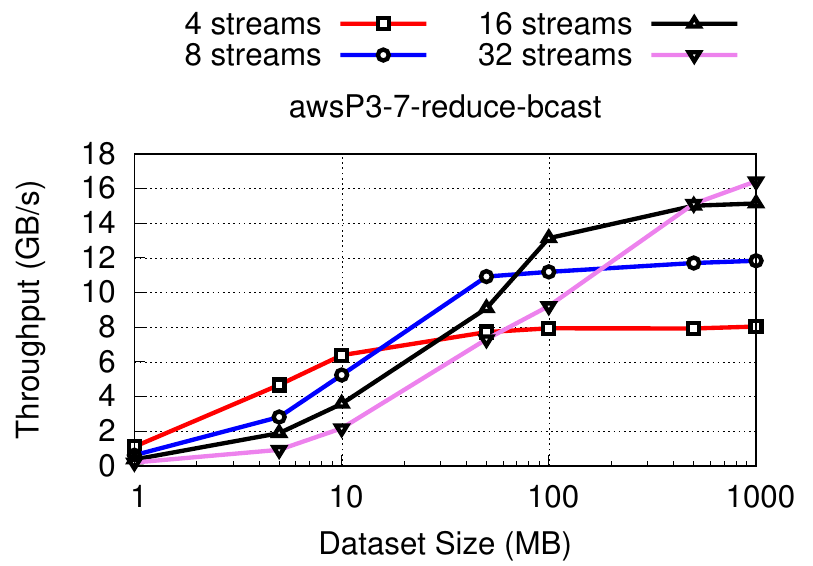}}
\subfigure[8 GPU chain forward]{\label{fig:awsP3-8-chain-f}
\includegraphics[width=0.32\textwidth]{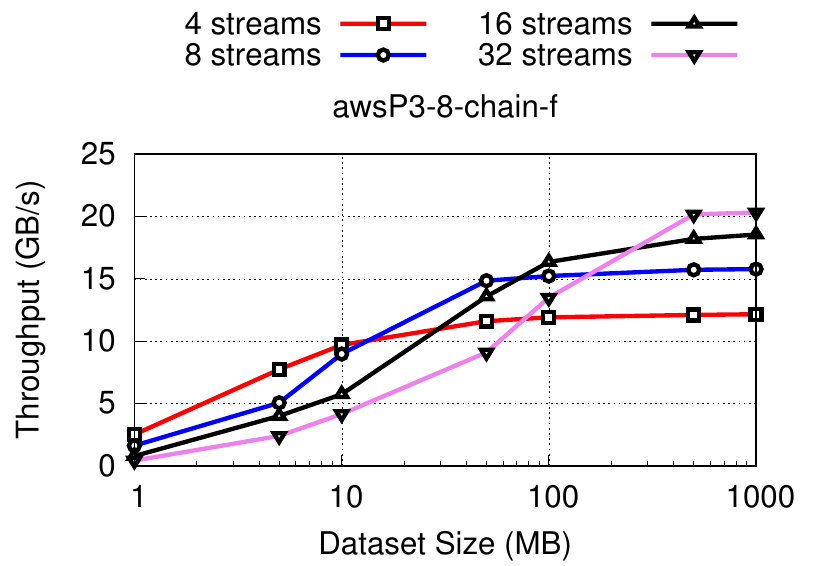}}
\subfigure[8 GPU chain reduce+forward]{\label{fig:awsP3-8-chain-af} 
\includegraphics[width=0.32\textwidth]{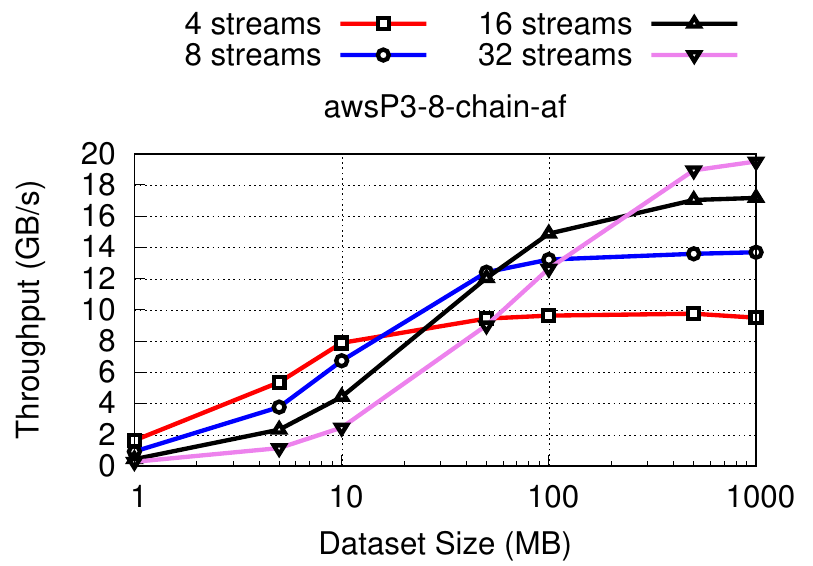}}
\subfigure[8 GPU chain reduce+bcast]{\label{fig:awsP3-8-reduce-bcast} 
\includegraphics[width=0.32\textwidth]{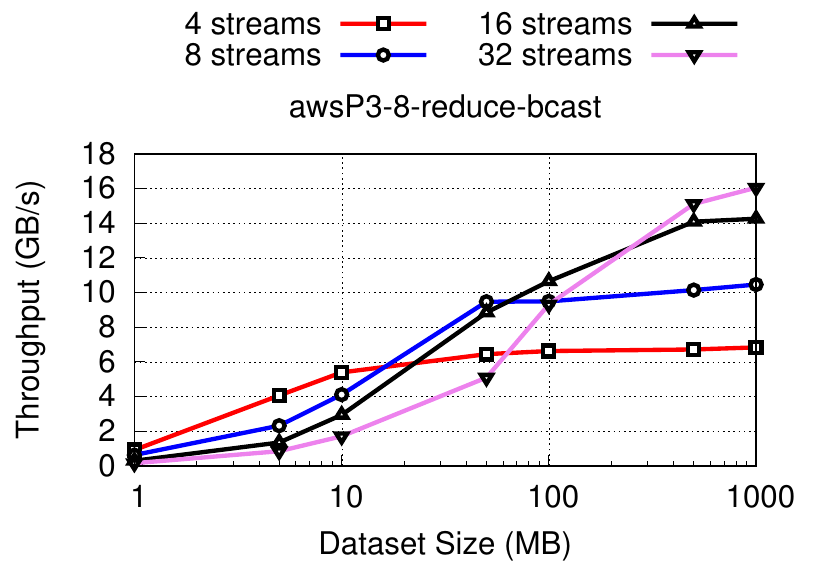}}
\vspace{-3mm}
\label{fig:aws-678-chain}
\caption{AWS 6,7,8 chain forward, reduce+forward, reduce-bcast}
\vspace{-3mm}
\end{figure*}
 
\begin{figure*}[h]
\centering
\subfigure[speedup in communication]{\label{fig:speedup-image1k-comm}
\includegraphics[width=0.8\textwidth]{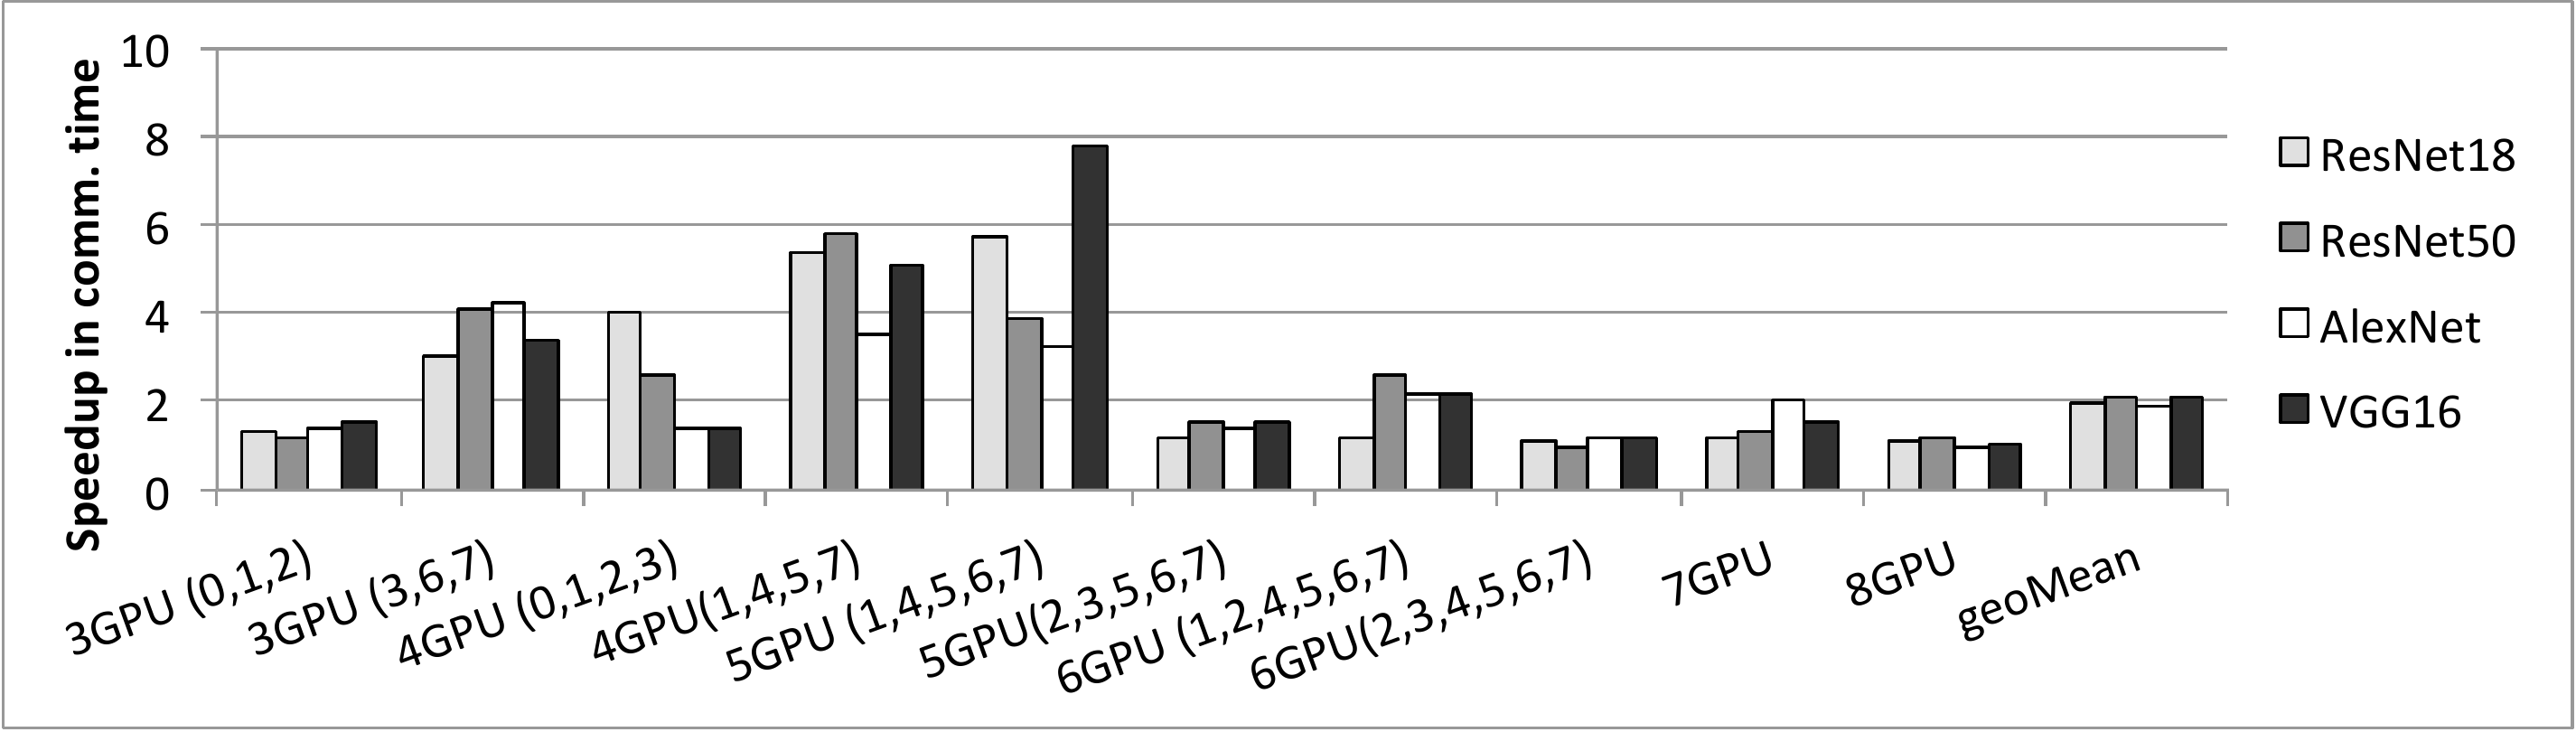}}
\subfigure[speedup in iteration]{\label{fig:speedup-image1k-iter} 
\includegraphics[width=0.8\textwidth]{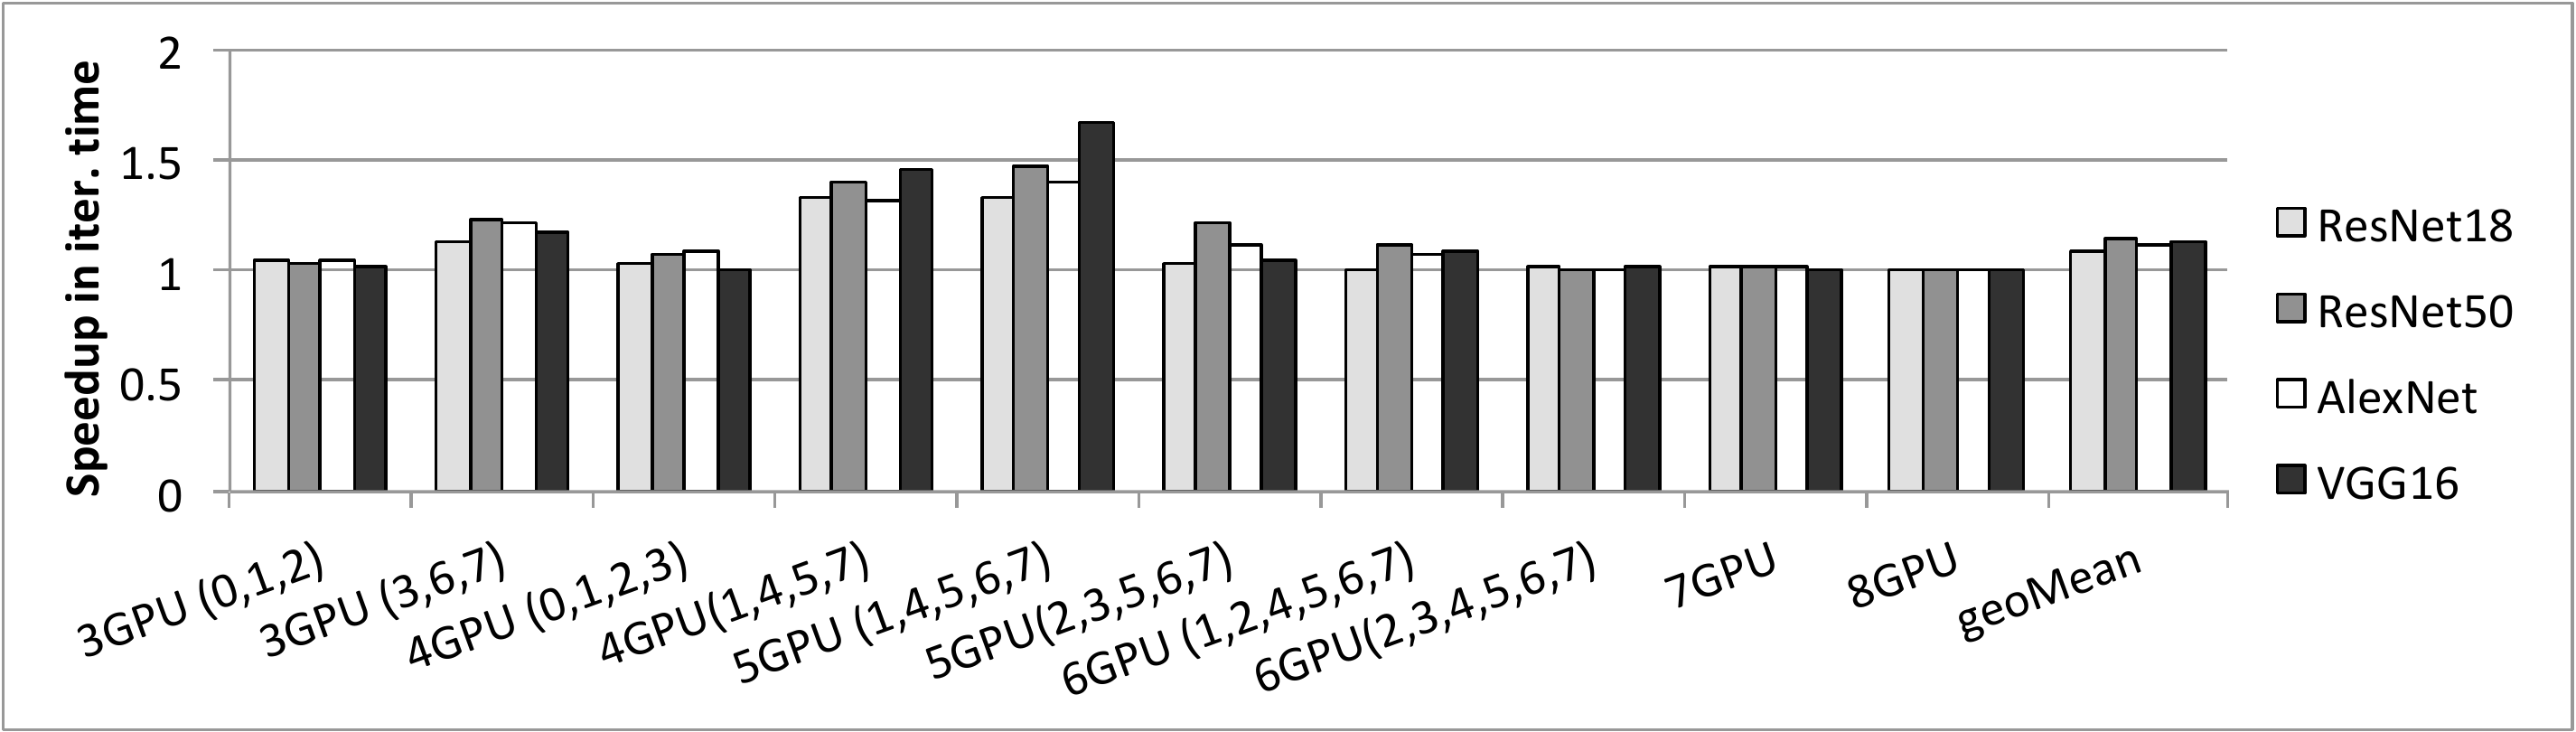}}
\vspace{-3mm}
\label{fig:speedup-image1k}
\caption{Speedup in communication and e2e iteration(ImageNet1K)}
\vspace{-3mm}
\end{figure*}
 
\begin{figure*}[h]
\centering
\subfigure[speedup in communication]{\label{fig:speedup-cifar10-comm}
\includegraphics[width=0.8\textwidth]{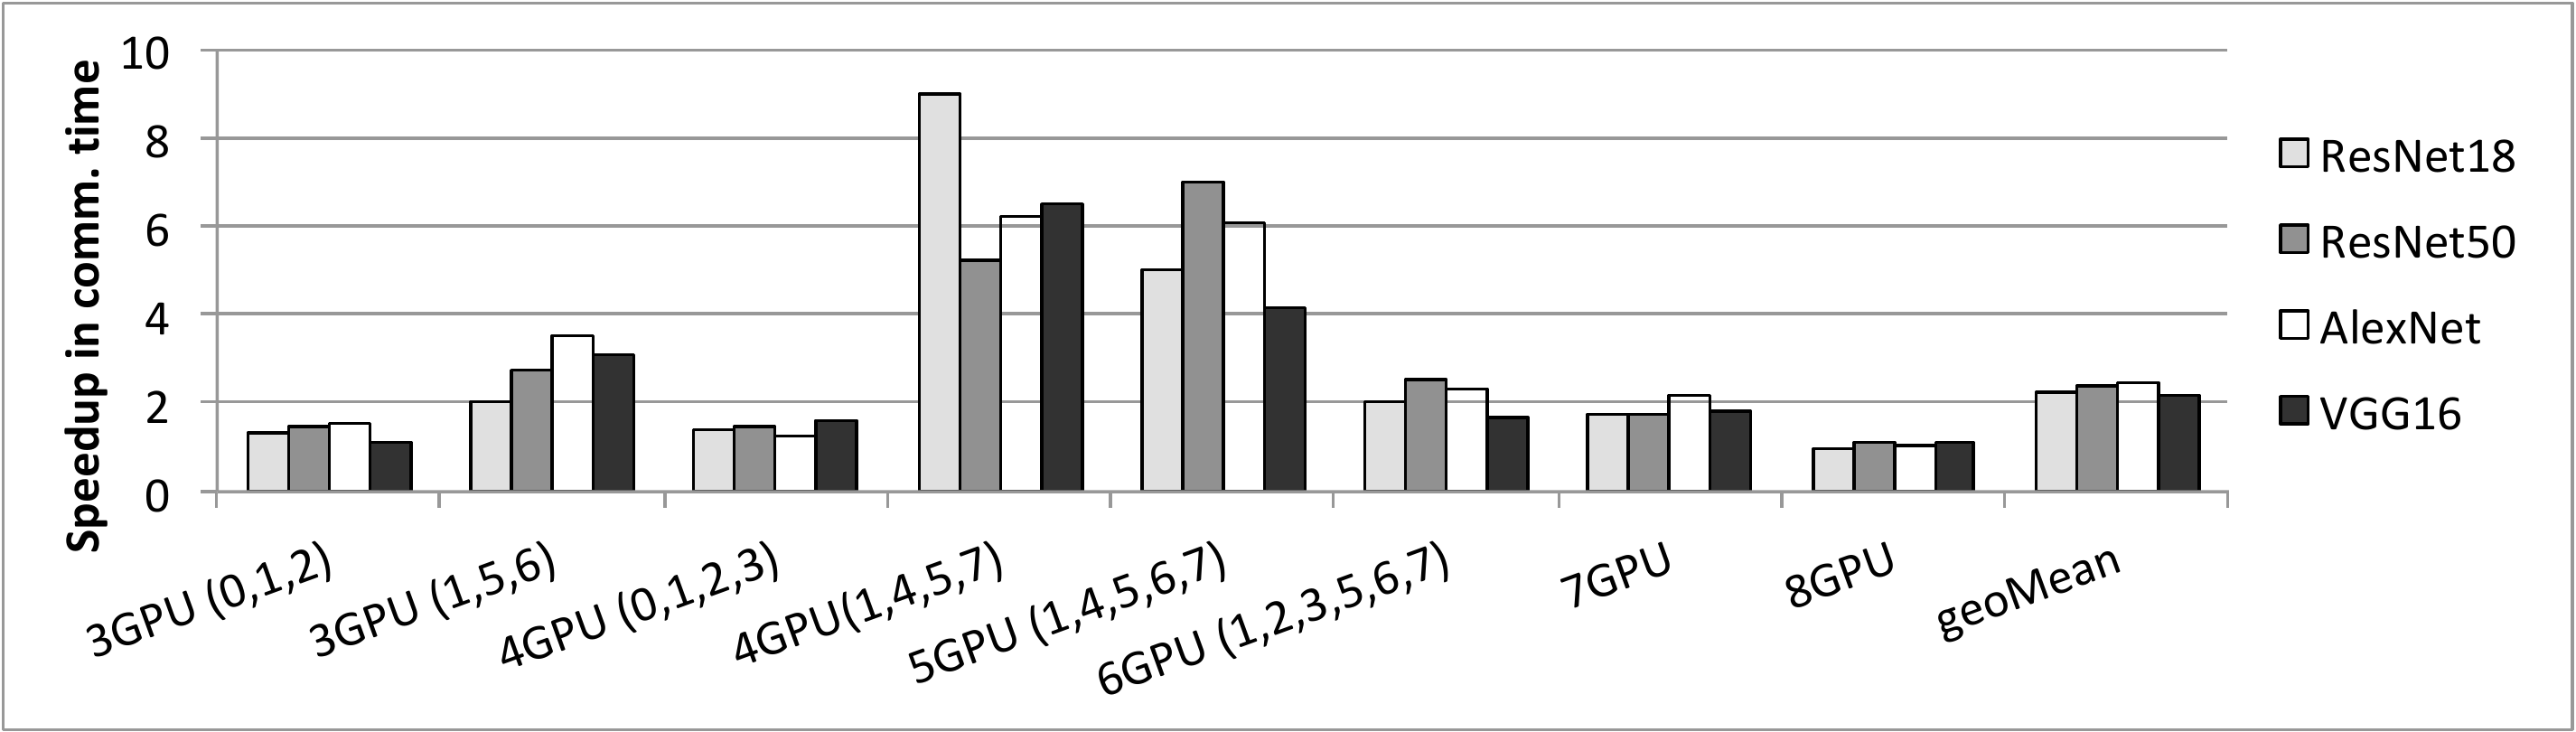}}
\subfigure[speedup in iteration]{\label{fig:speedup-cifar10-iter} 
\includegraphics[width=0.8\textwidth]{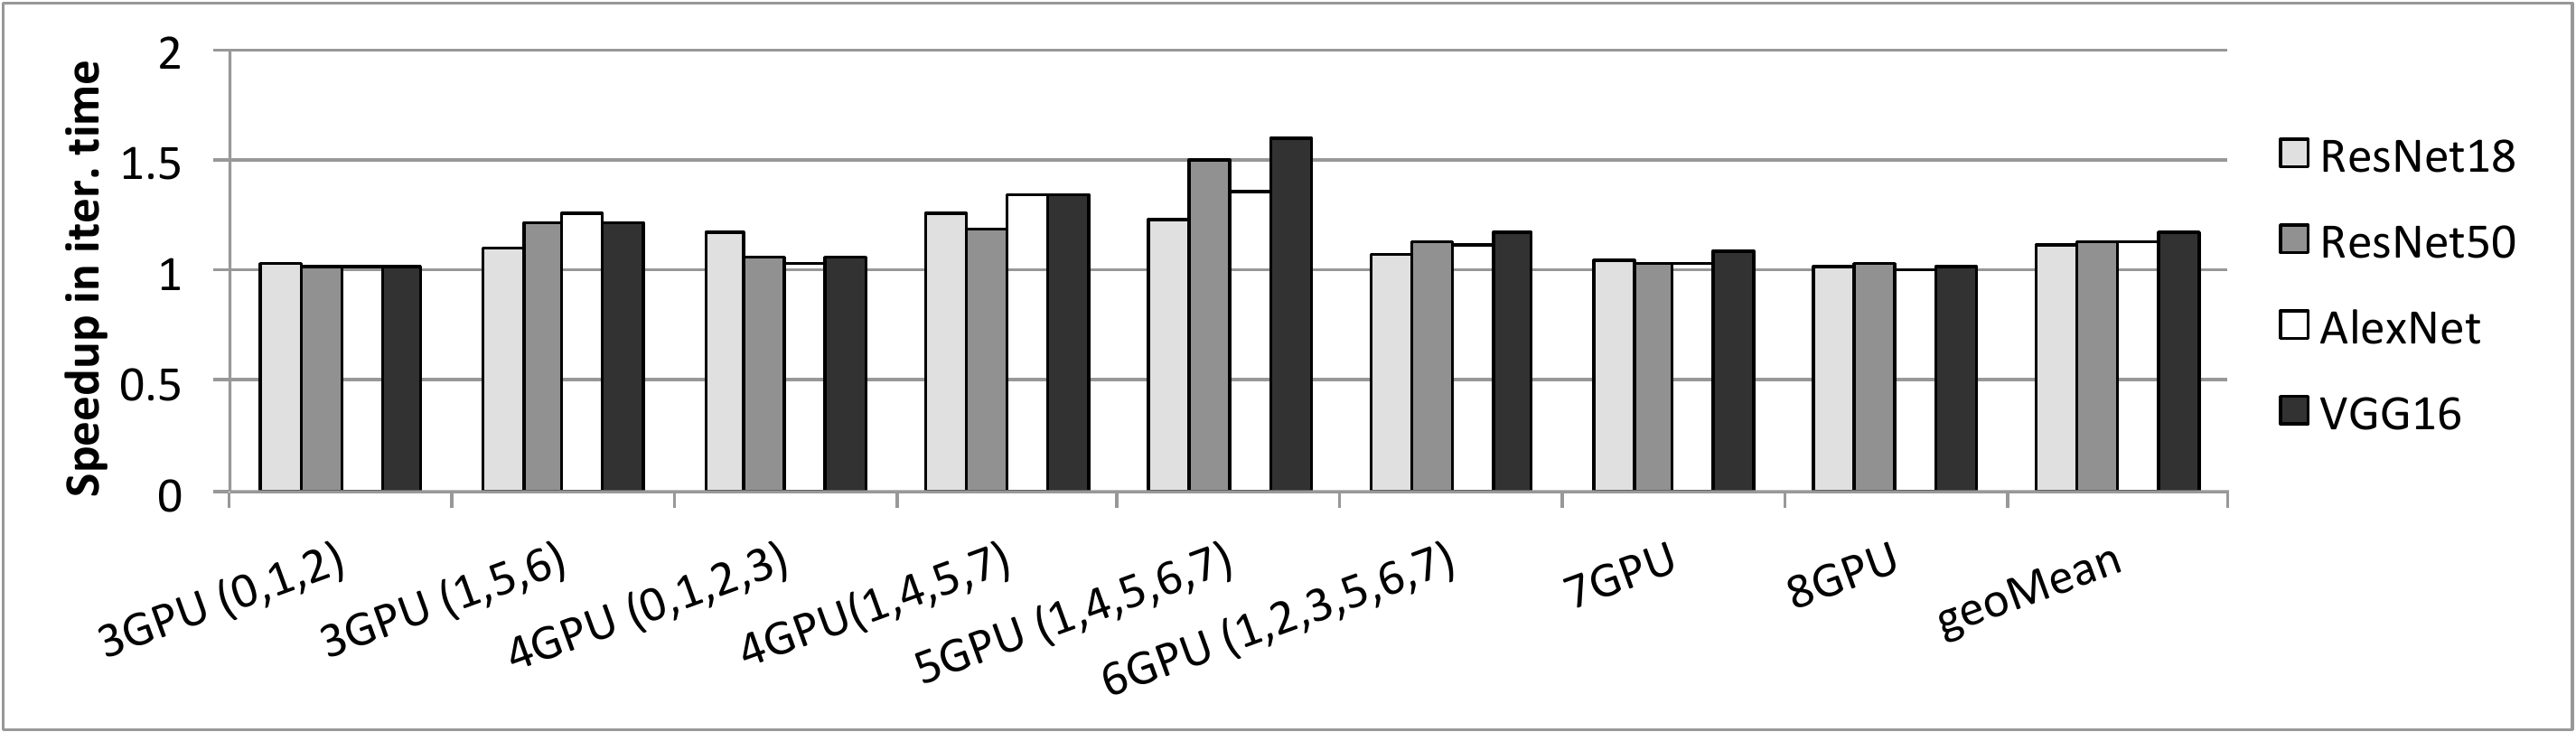}}
\vspace{-3mm}
\label{fig:speedup-cifar10}
\caption{Speedup in communication and e2e iteration(CIFAR10)}
\vspace{-3mm}
\end{figure*} 

\clearpage
\newpage
\subsection{HGX-1-P100}

\begin{figure*}[h]
\centering
\subfigure[Fan-in forward throughput]{\label{fig:msr-1-fan-in-f}
\includegraphics[width=0.32\textwidth]{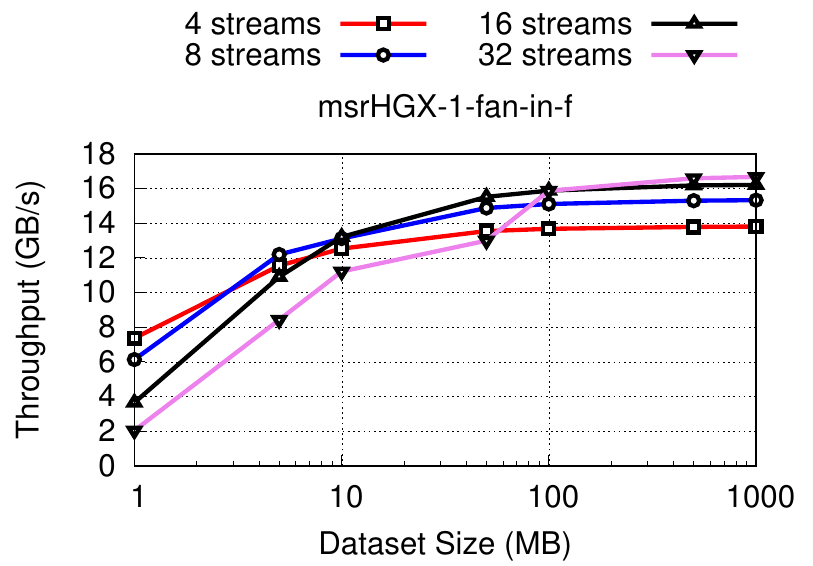}}
\subfigure[Fan-in reduce+forward throughput]{\label{fig:msr-1-fan-in-af} 
\includegraphics[width=0.32\textwidth]{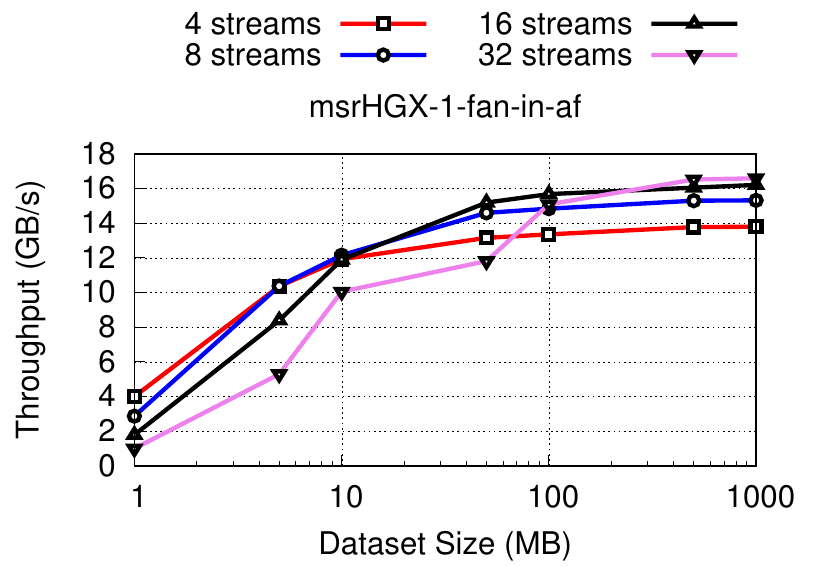}}
\subfigure[Fan-out forward throughput]{\label{fig:msr-1-fan-out-f} 
\includegraphics[width=0.32\textwidth]{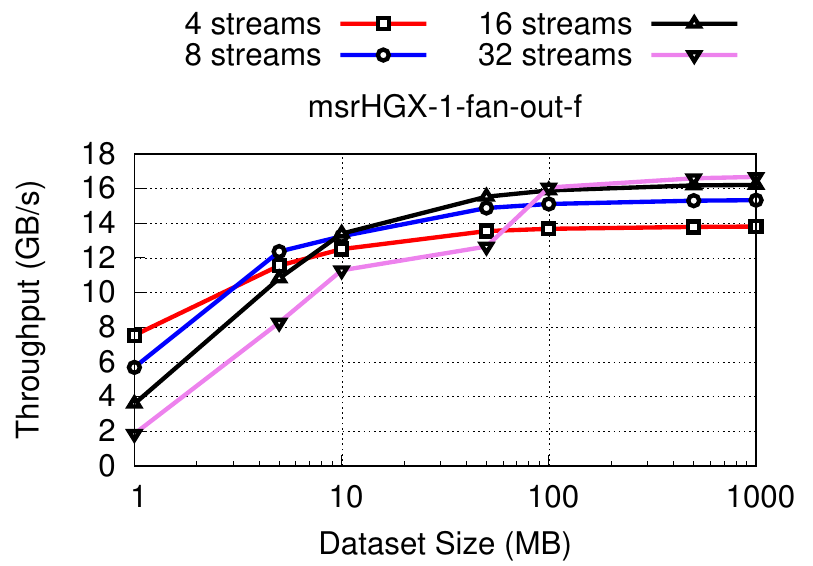}}
\subfigure[Fan-in forward throughput]{\label{fig:msr-2-fan-in-f}
\includegraphics[width=0.32\textwidth]{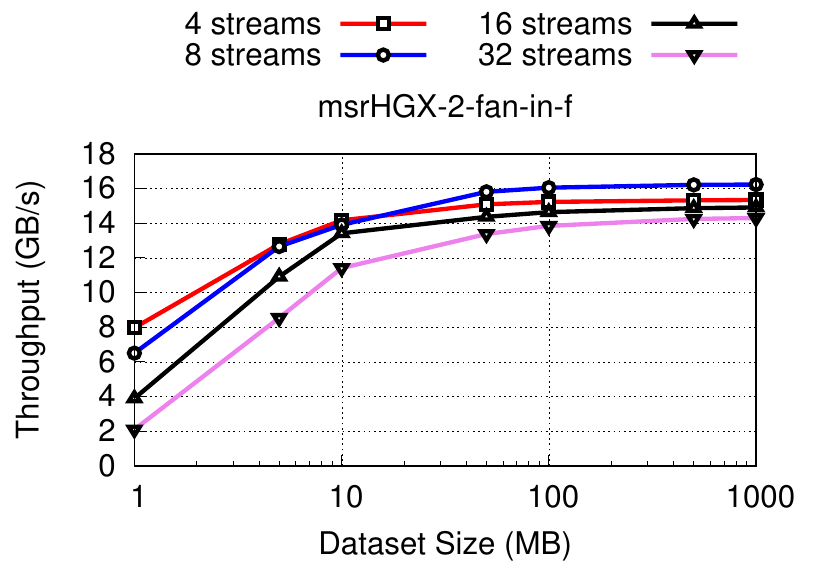}}
\subfigure[Fan-in reduce+forward throughput]{\label{fig:msr-2-fan-in-af} 
\includegraphics[width=0.32\textwidth]{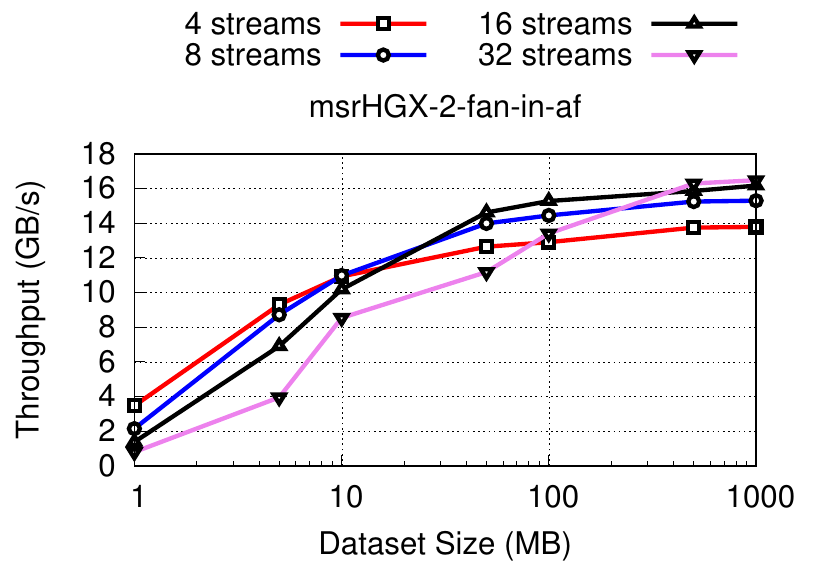}}
\subfigure[Fan-out forward throughput]{\label{fig:msr-2-fan-out-f} 
\includegraphics[width=0.32\textwidth]{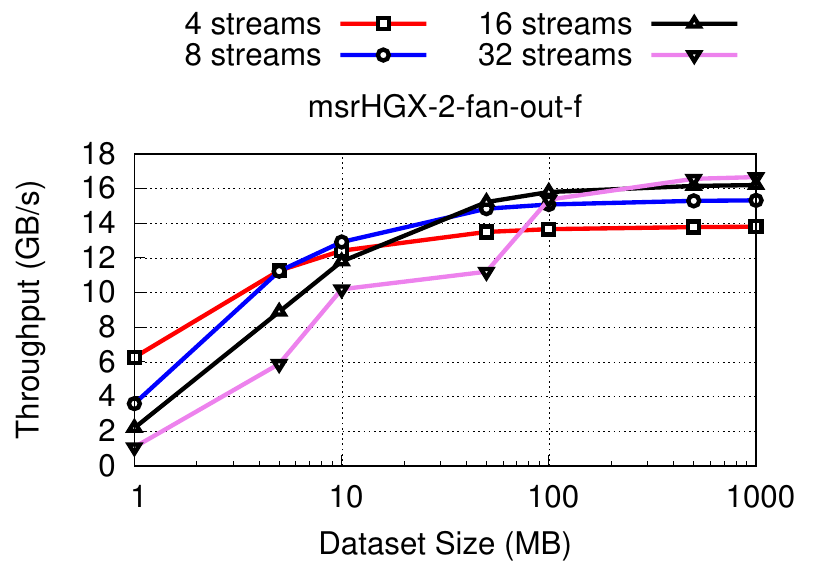}}
\subfigure[Fan-in forward throughput]{\label{fig:msr-3-fan-in-f}
\includegraphics[width=0.32\textwidth]{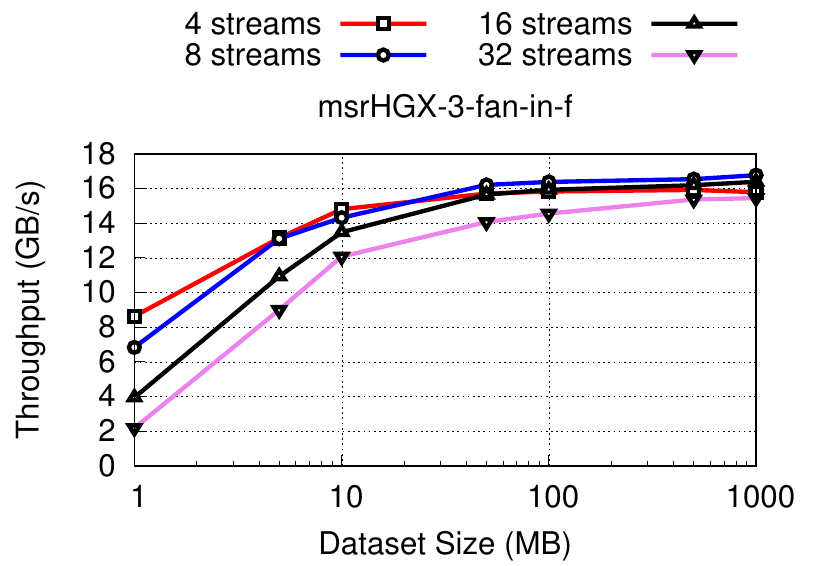}}
\subfigure[Fan-in reduce+forward throughput]{\label{fig:msr-3-fan-in-af} 
\includegraphics[width=0.32\textwidth]{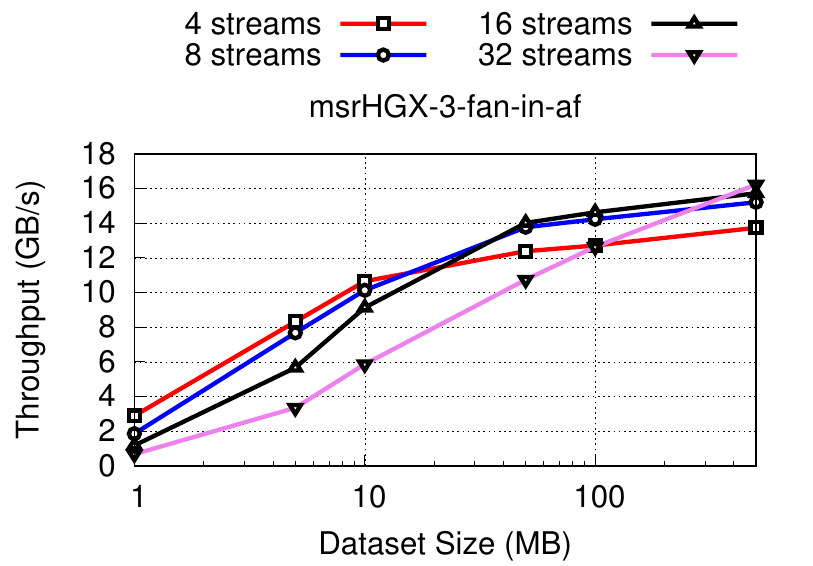}}
\subfigure[Fan-out forward throughput]{\label{fig:msr-3-fan-out-f} 
\includegraphics[width=0.32\textwidth]{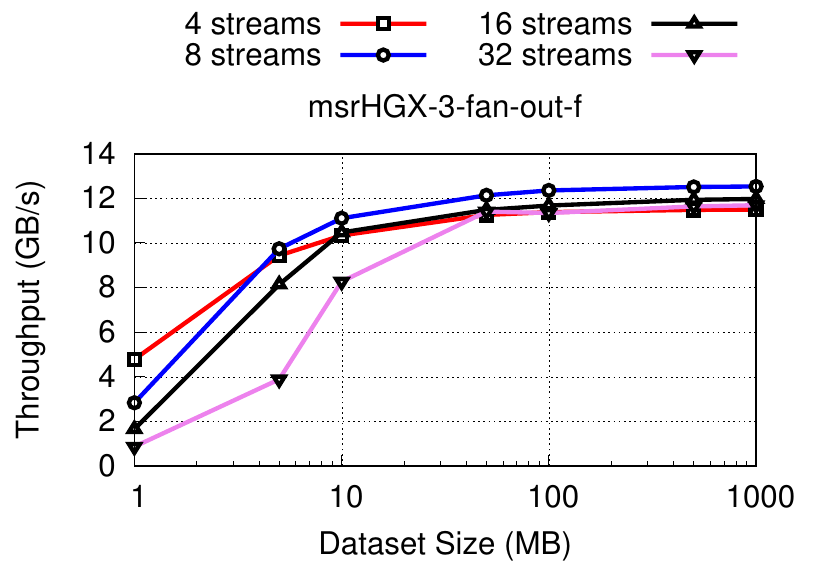}}
\vspace{-3mm}
\label{fig:msr-fanin-fanout}
\caption{MSR Fan-in forward, add+forward, Fan-out forward}
\vspace{-3mm}
\end{figure*}

\begin{figure*}[h]
\centering
\subfigure[MIMO]{\label{fig:msr-2i2o-af}
\includegraphics[width=0.32\textwidth]{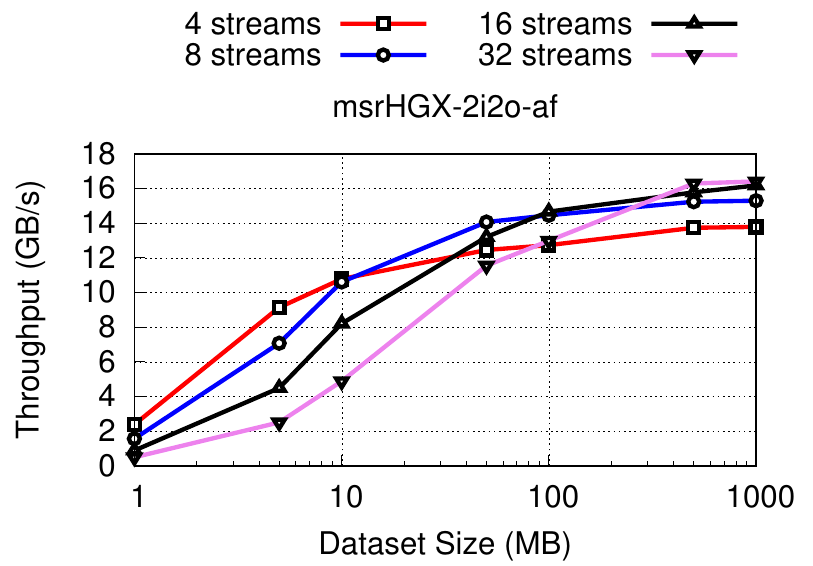}}
\subfigure[MCA]{\label{fig:msr-mc-af} 
\includegraphics[width=0.32\textwidth]{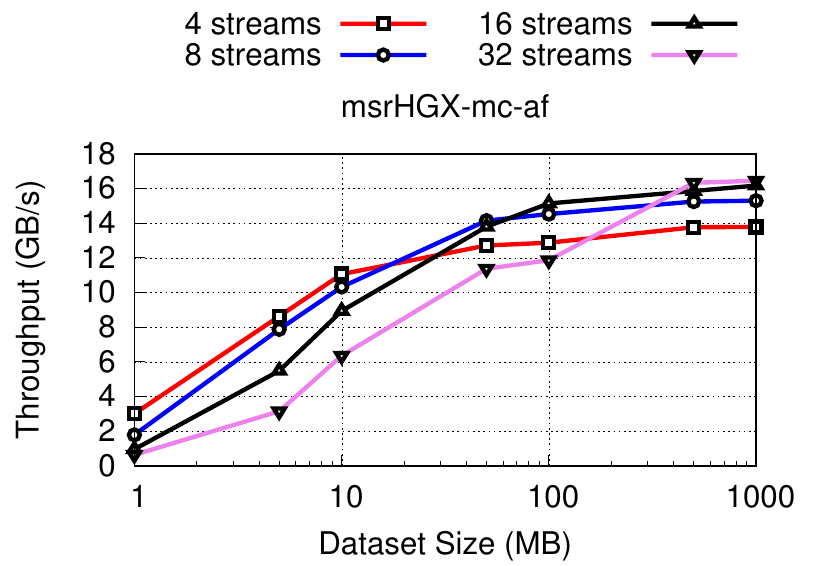}}
\vspace{-3mm}
\label{fig:msr-mimo-mca}
\caption{MSR MIMO MCA}
\vspace{-3mm}
\end{figure*}

\begin{figure*}[h]
\centering
\subfigure[3 GPU chain forward]{\label{fig:msr-3-chain-f}
\includegraphics[width=0.32\textwidth]{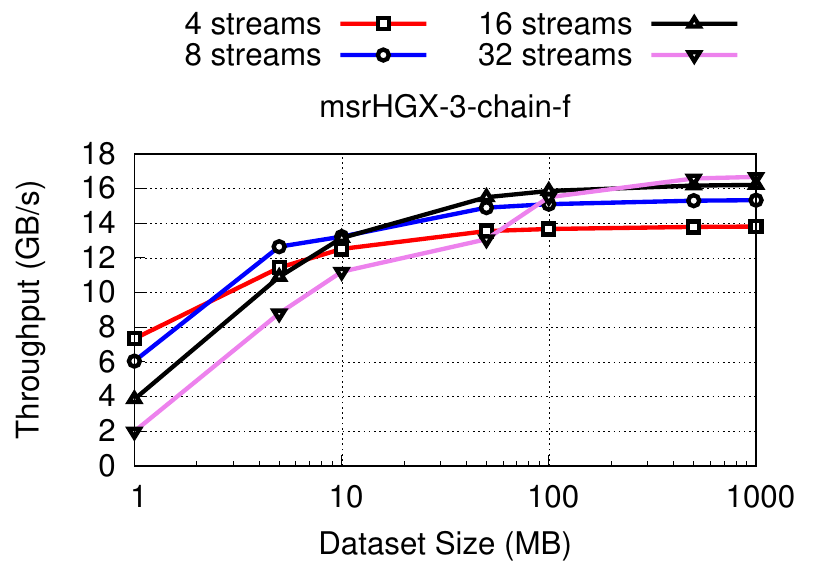}}
\subfigure[3 GPU chain reduce+forward]{\label{fig:msr-3-chain-af} 
\includegraphics[width=0.32\textwidth]{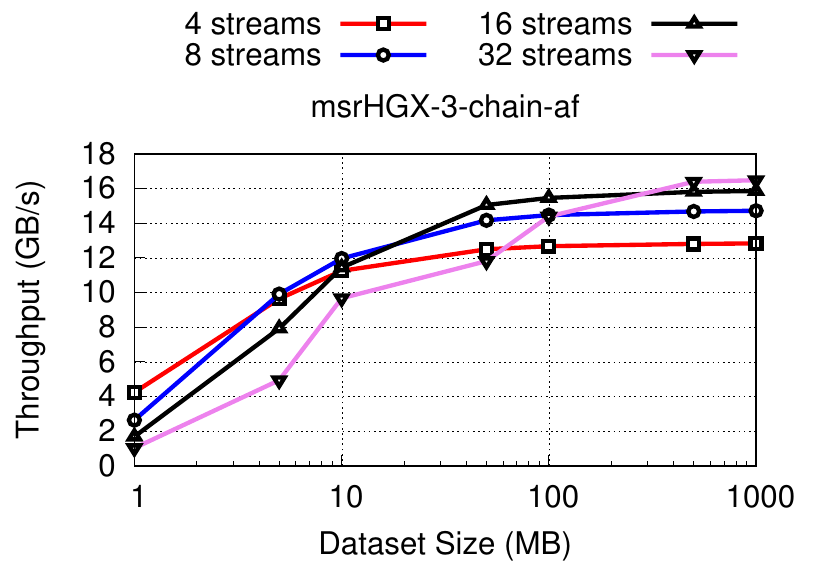}}
\subfigure[3 GPU chain reduce+bcast]{\label{fig:msr-3-reduce-bcast} 
\includegraphics[width=0.32\textwidth]{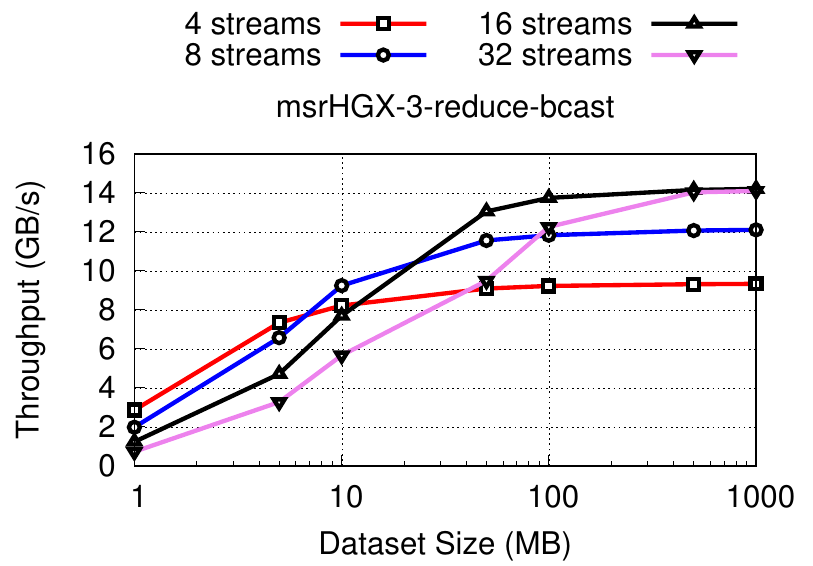}}
\subfigure[4 GPU chain forward]{\label{fig:msr-4-chain-f}
\includegraphics[width=0.32\textwidth]{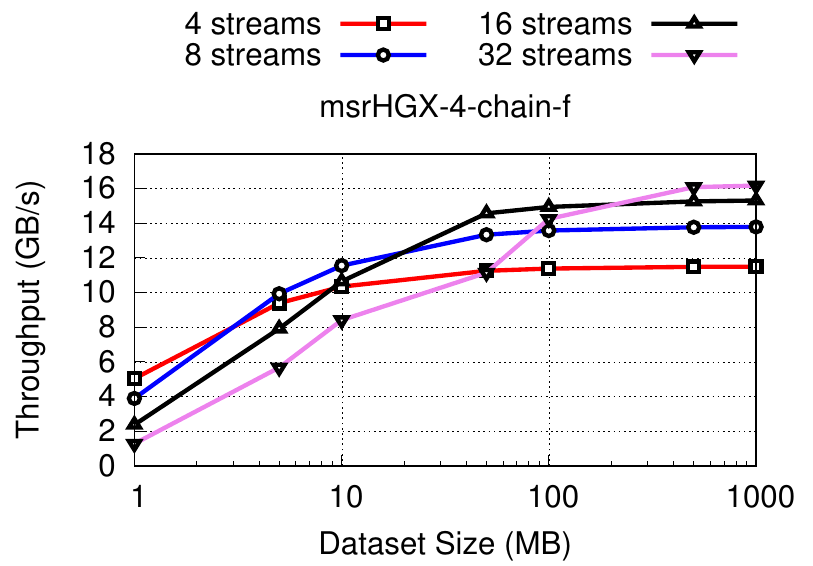}}
\subfigure[4 GPU chain reduce+forward]{\label{fig:msr-4-chain-af} 
\includegraphics[width=0.32\textwidth]{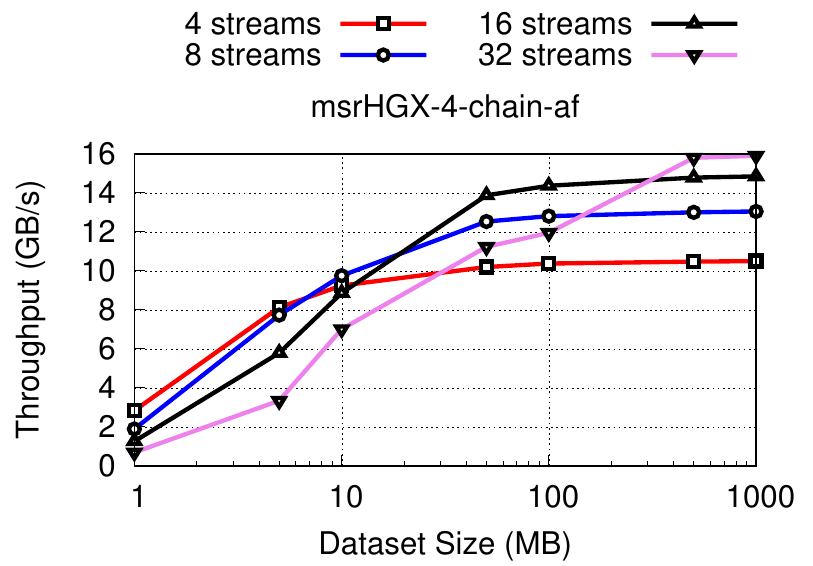}}
\subfigure[4 GPU chain reduce+bcast]{\label{fig:msr-4-reduce-bcast} 
\includegraphics[width=0.32\textwidth]{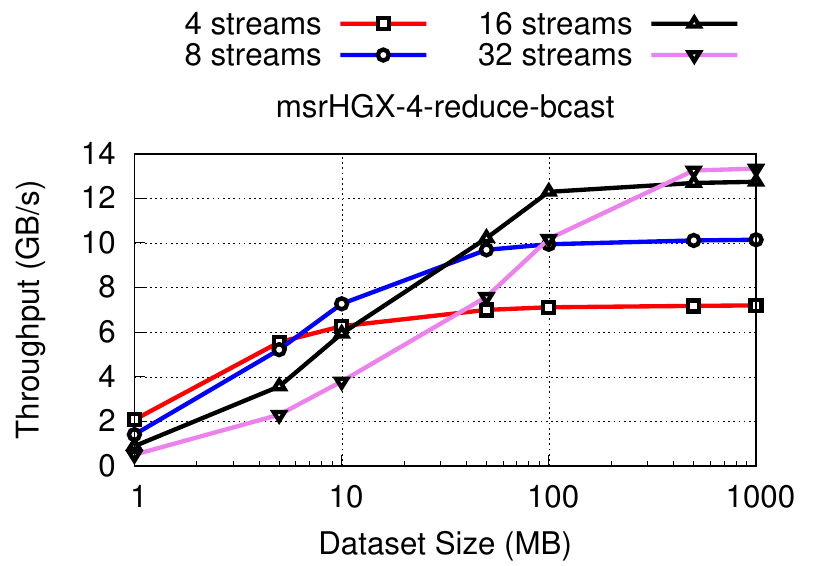}}
\subfigure[5 GPU chain forward]{\label{fig:msr-5-chain-f}
\includegraphics[width=0.32\textwidth]{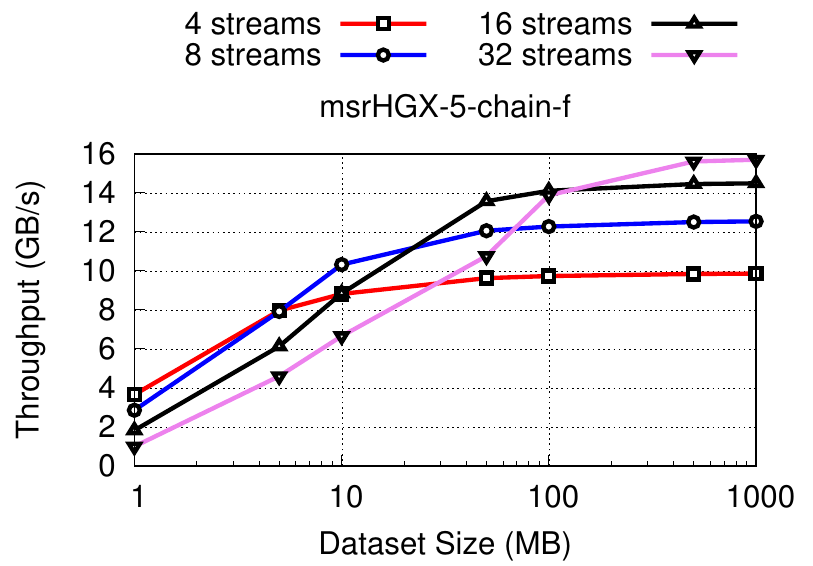}}
\subfigure[5 GPU chain reduce+forward]{\label{fig:msr-5-chain-af} 
\includegraphics[width=0.32\textwidth]{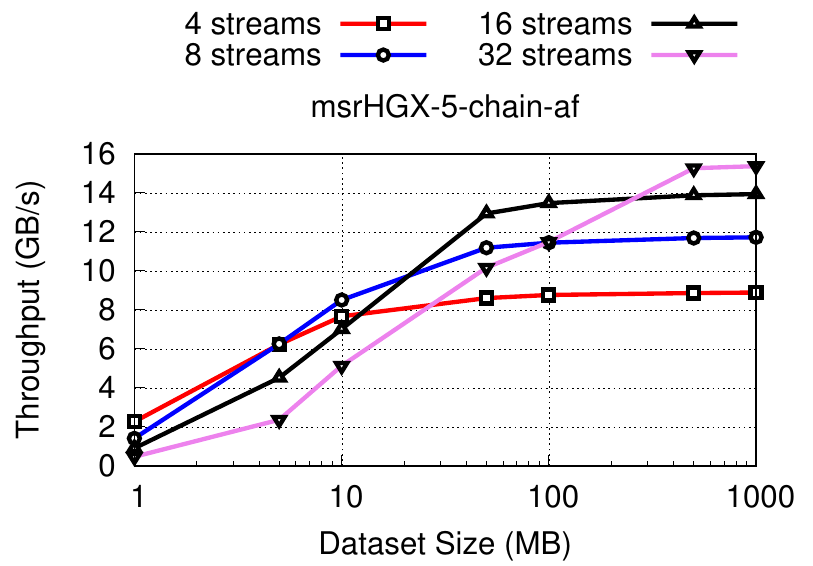}}
\subfigure[5 GPU chain reduce+bcast]{\label{fig:msr-5-reduce-bcast} 
\includegraphics[width=0.32\textwidth]{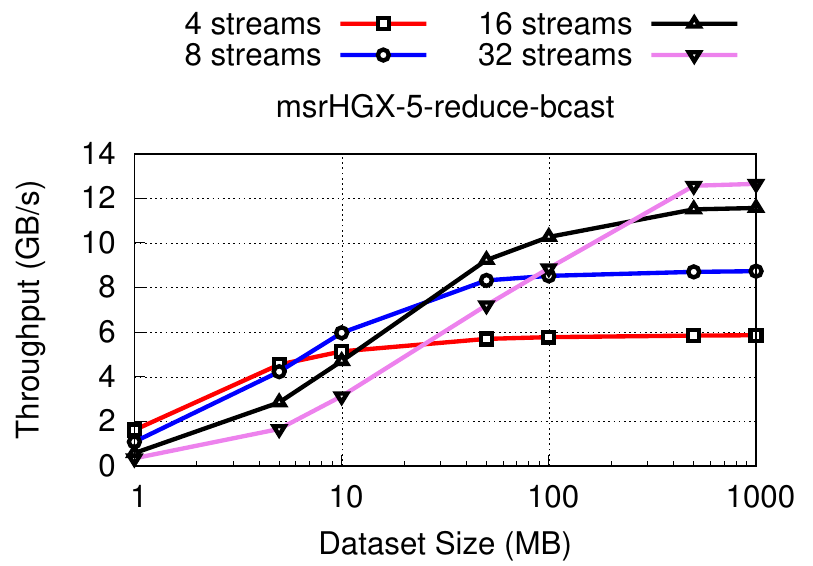}}
\vspace{-3mm}
\label{fig:msr-345-chain}
\caption{MSR 3,4,5 chain forward, reduce+forward, reduce-bcast}
\vspace{-3mm}
\end{figure*}

\begin{figure*}[h]
\centering
\subfigure[6 GPU chain forward]{\label{fig:msr-6-chain-f}
\includegraphics[width=0.32\textwidth]{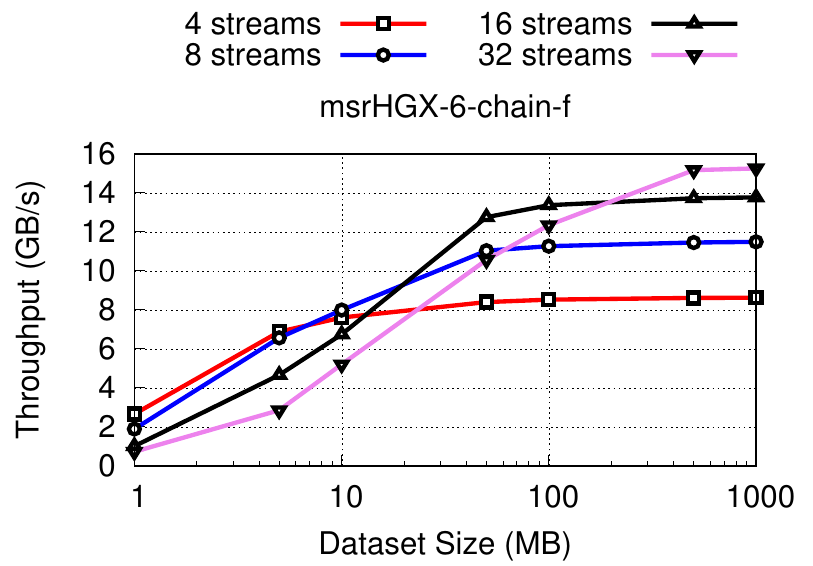}}
\subfigure[6 GPU chain reduce+forward]{\label{fig:msr-6-chain-af} 
\includegraphics[width=0.32\textwidth]{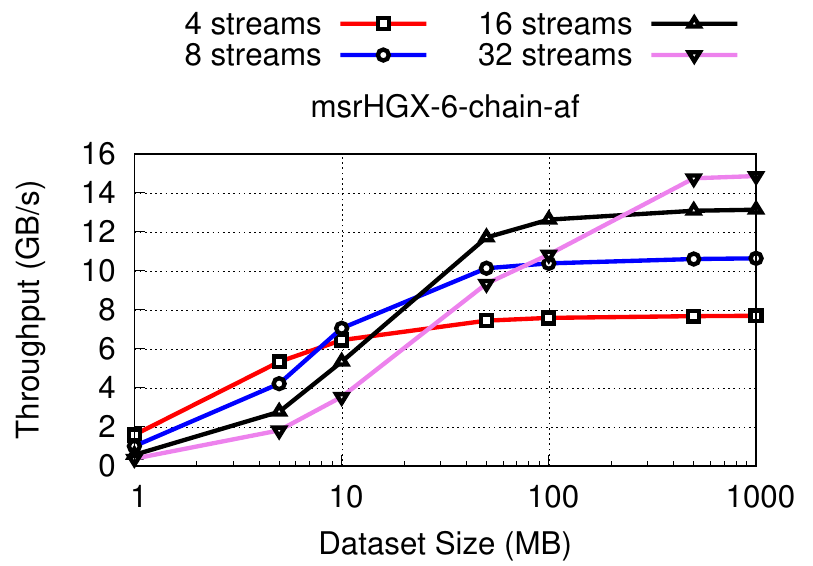}}
\subfigure[6 GPU chain reduce+bcast]{\label{fig:msr-6-reduce-bcast} 
\includegraphics[width=0.32\textwidth]{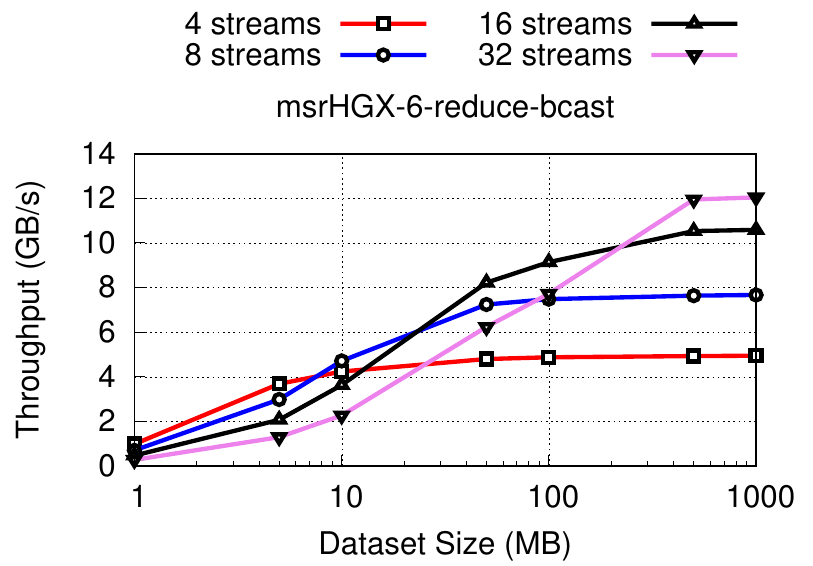}}

\subfigure[7 GPU chain forward]{\label{fig:msr-7-chain-f}
\includegraphics[width=0.32\textwidth]{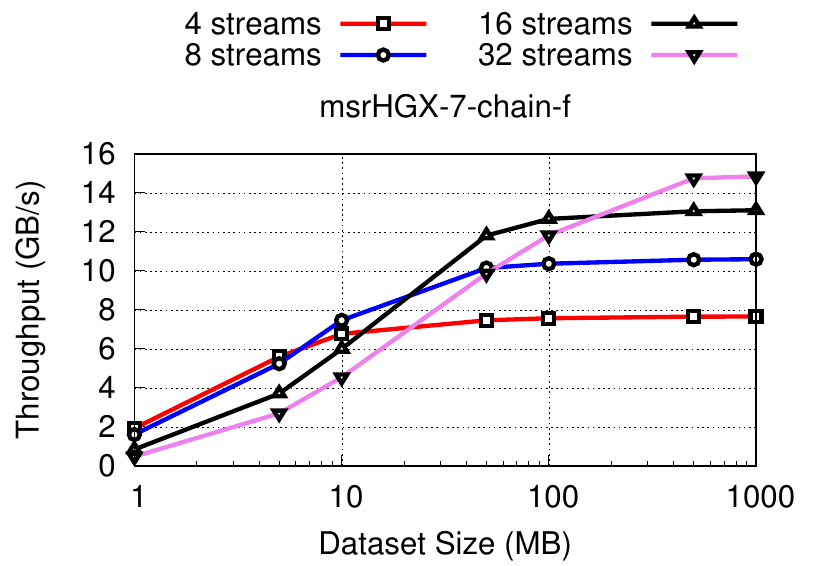}}
\subfigure[7 GPU chain reduce+forward]{\label{fig:msr-7-chain-af} 
\includegraphics[width=0.32\textwidth]{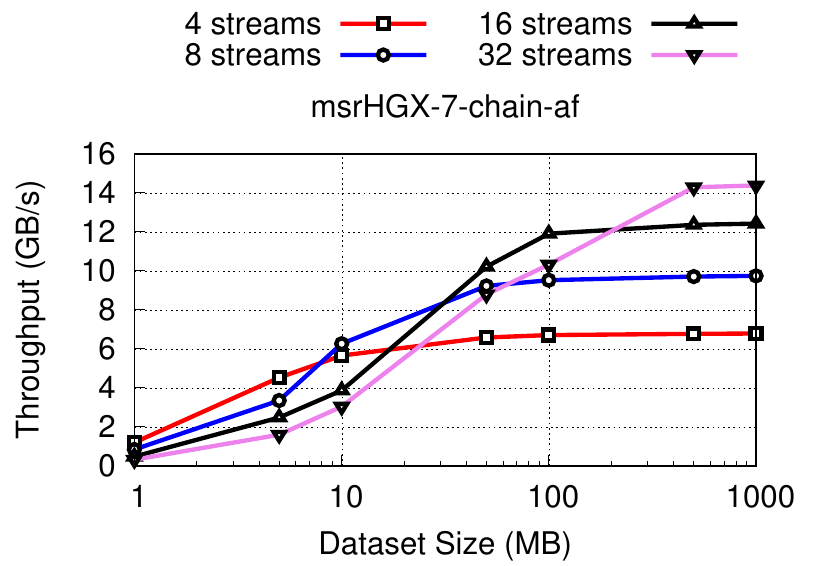}}
\subfigure[7 GPU chain reduce+bcast]{\label{fig:msr-7-reduce-bcast} 
\includegraphics[width=0.32\textwidth]{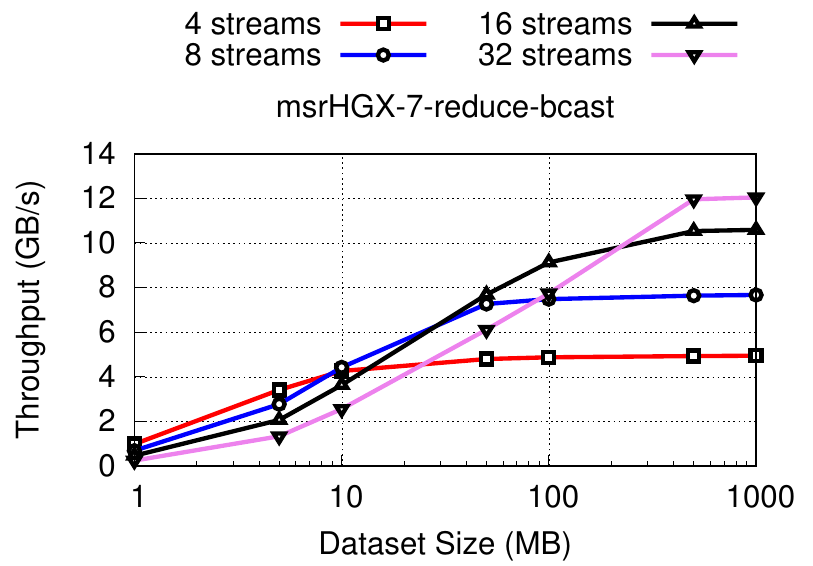}}

\subfigure[8 GPU chain forward]{\label{fig:msr-8-chain-f}
\includegraphics[width=0.32\textwidth]{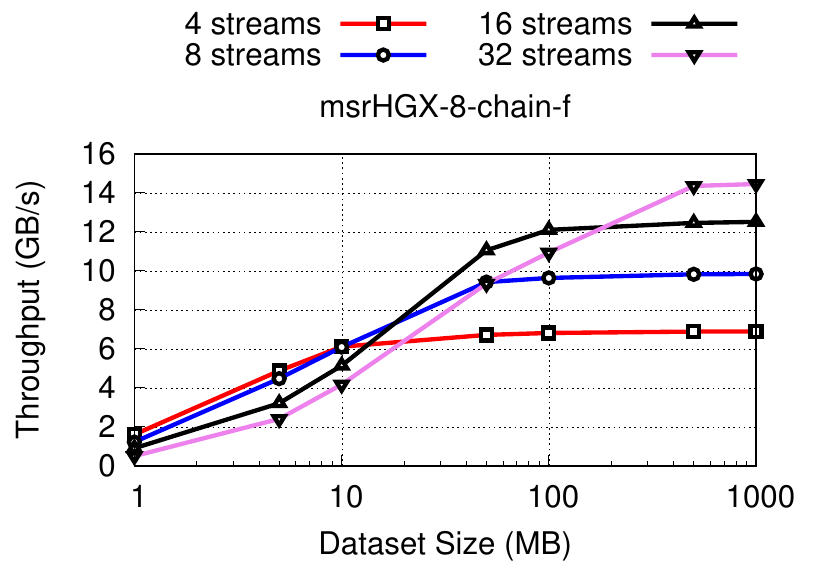}}
\subfigure[8 GPU chain reduce+forward]{\label{fig:msr-8-chain-af} 
\includegraphics[width=0.32\textwidth]{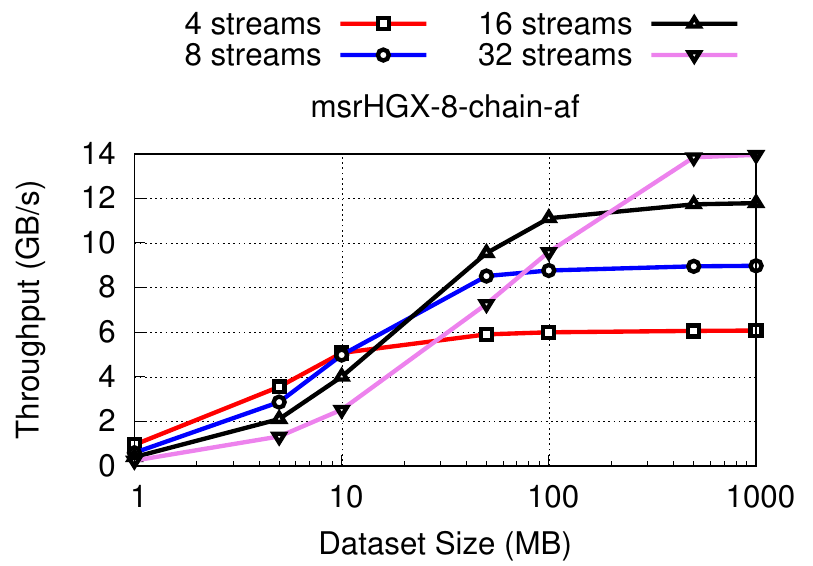}}
\subfigure[8 GPU chain reduce+bcast]{\label{fig:msr-8-reduce-bcast} 
\includegraphics[width=0.32\textwidth]{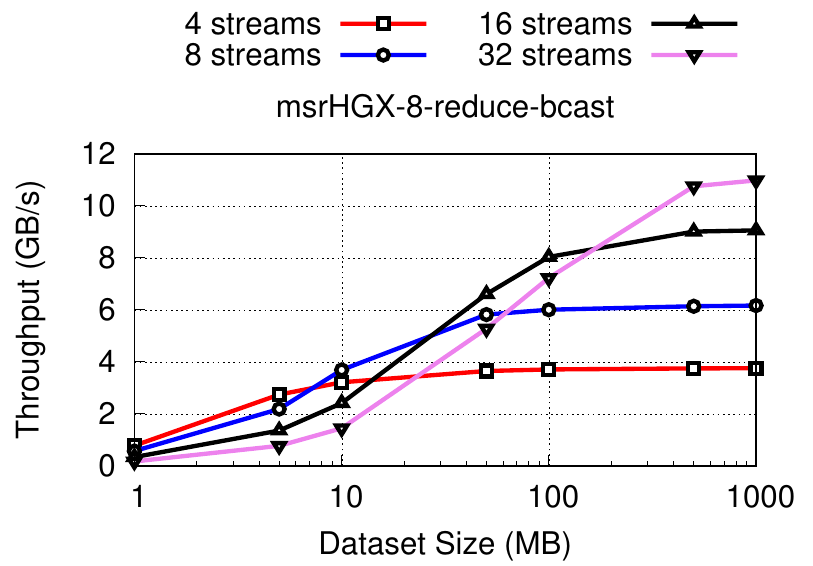}}
\vspace{-3mm}
\label{fig:msr-678-chain}
\caption{MSR 6,7,8 chain forward, reduce+forward, reduce-bcast}
\vspace{-3mm}
\end{figure*}

\clearpage
\newpage

\subsection{DGX-1-P100}

\begin{figure*}[h]
\centering
\subfigure[Fan-in forward throughput]{\label{fig:msr-dgx-p100-1-fan-in-f}
\includegraphics[width=0.32\textwidth]{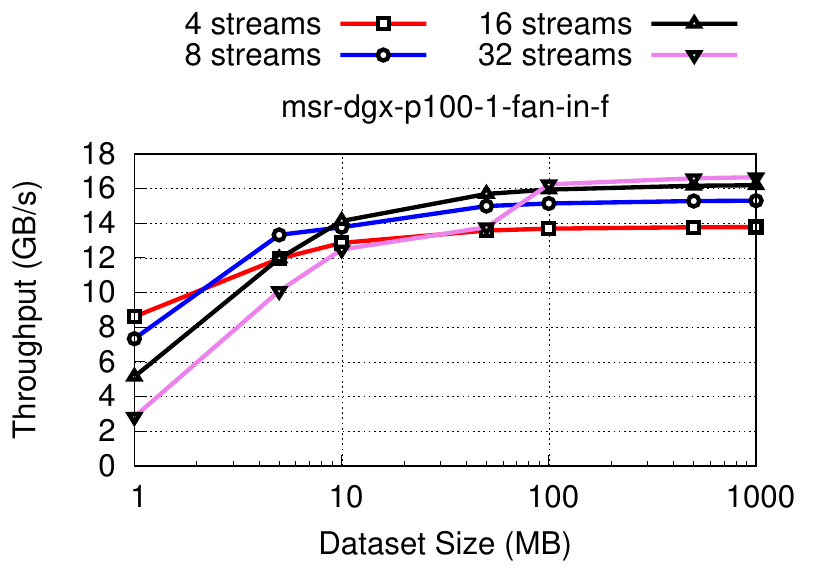}}
\subfigure[Fan-in reduce+forward throughput]{\label{fig:msr-dgx-p100-1-fan-in-af} 
\includegraphics[width=0.32\textwidth]{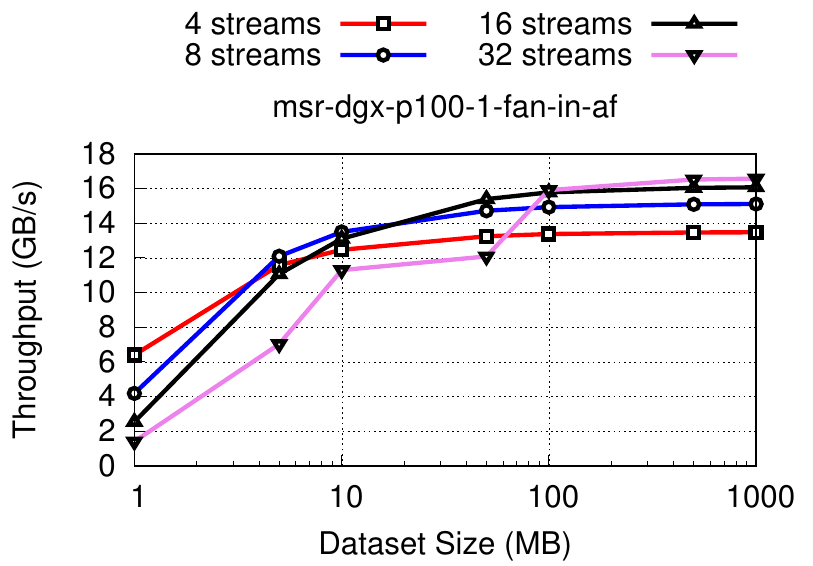}}
\subfigure[Fan-out forward throughput]{\label{fig:msr-dgx-p100-1-fan-out-f} 
\includegraphics[width=0.32\textwidth]{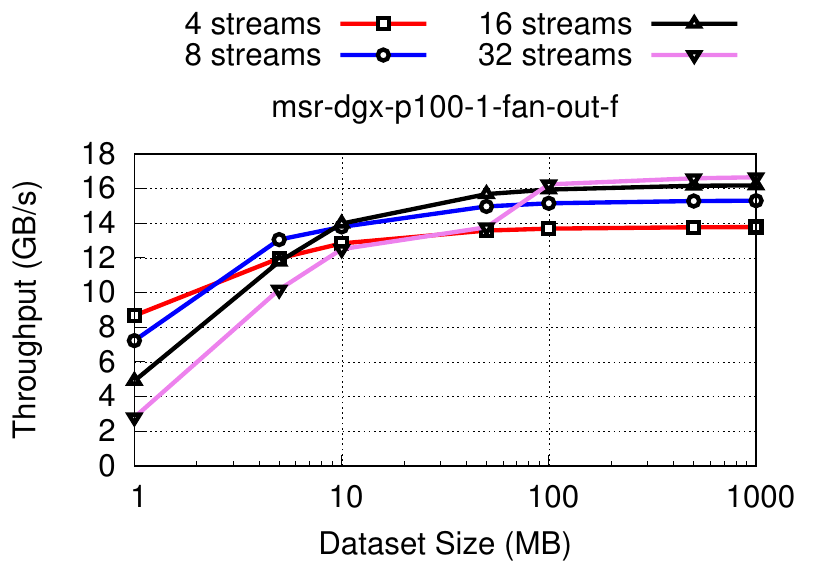}}
\subfigure[Fan-in forward throughput]{\label{fig:msr-dgx-p100-2-fan-in-f}
\includegraphics[width=0.32\textwidth]{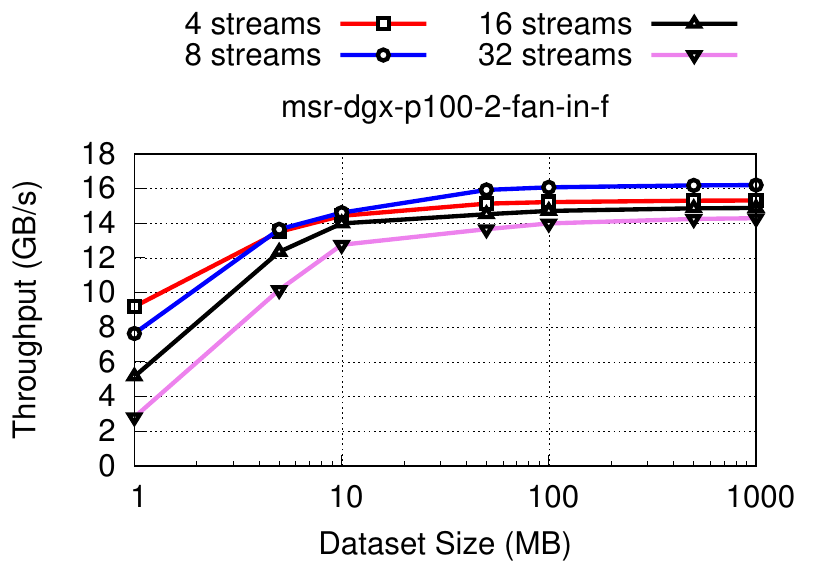}}
\subfigure[Fan-in reduce+forward throughput]{\label{fig:msr-dgx-p100-2-fan-in-af} 
\includegraphics[width=0.32\textwidth]{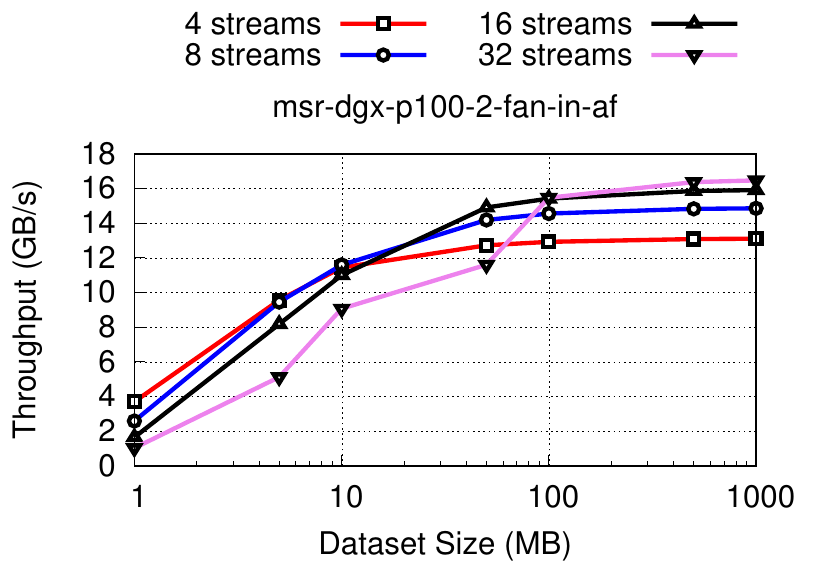}}
\subfigure[Fan-out forward throughput]{\label{fig:msr-dgx-p100-2-fan-out-f} 
\includegraphics[width=0.32\textwidth]{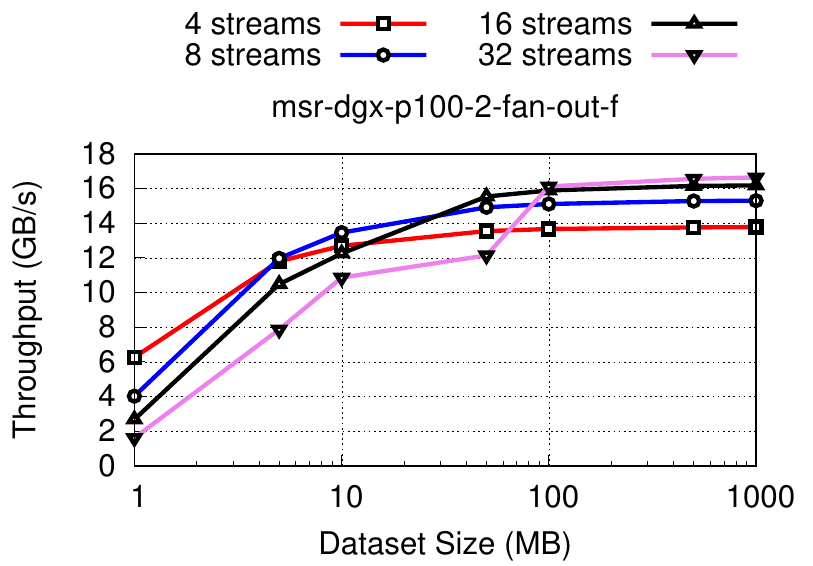}}
\subfigure[Fan-in forward throughput]{\label{fig:msr-dgx-p100-3-fan-in-f}
\includegraphics[width=0.32\textwidth]{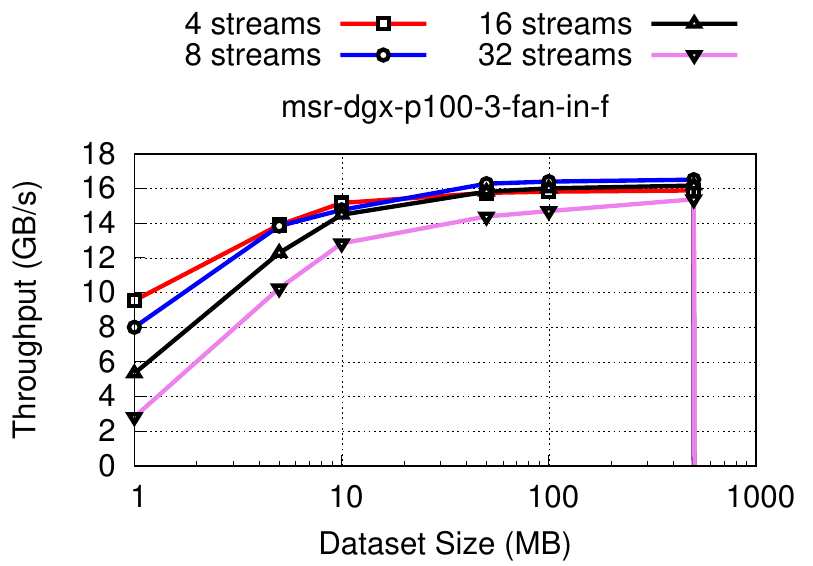}}
\subfigure[Fan-in reduce+forward throughput]{\label{fig:msr-dgx-p100-3-fan-in-af} 
\includegraphics[width=0.32\textwidth]{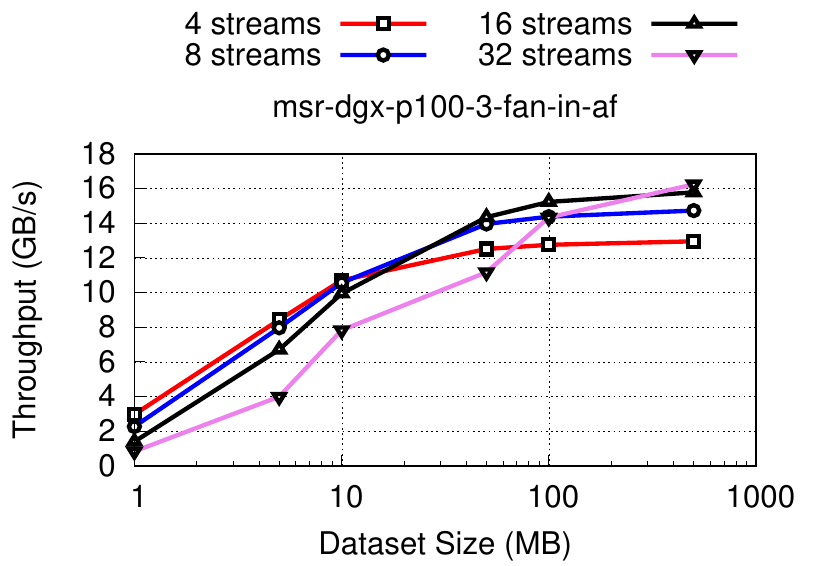}}
\subfigure[Fan-out forward throughput]{\label{fig:msr-dgx-p100-3-fan-out-f} 
\includegraphics[width=0.32\textwidth]{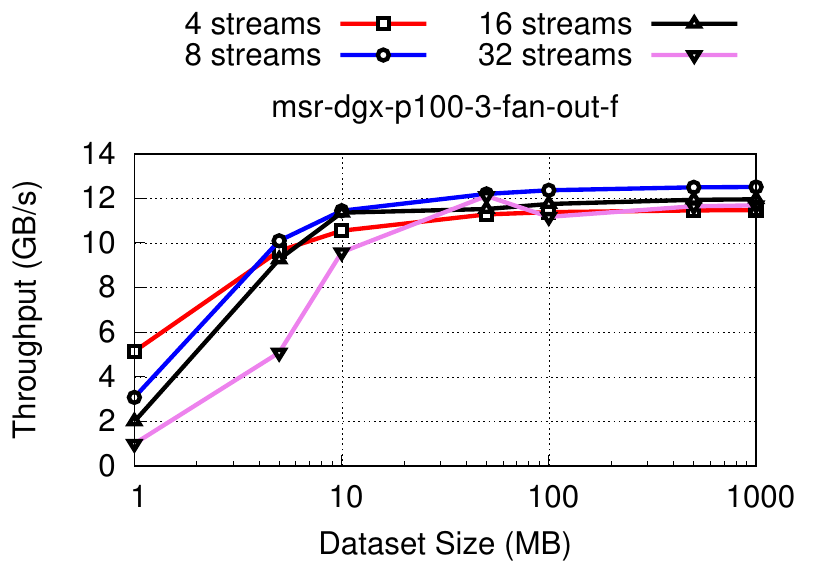}}
\vspace{-3mm}
\label{fig:msr-dgx-p100-fanin-fanout}
\caption{msr-dgx-p100 Fan-in forward, add+forward, Fan-out forward}
\vspace{-3mm}
\end{figure*}

\begin{figure*}[h]
\centering
\subfigure[MIMO]{\label{fig:msr-dgx-p100-2i2o-af}
\includegraphics[width=0.32\textwidth]{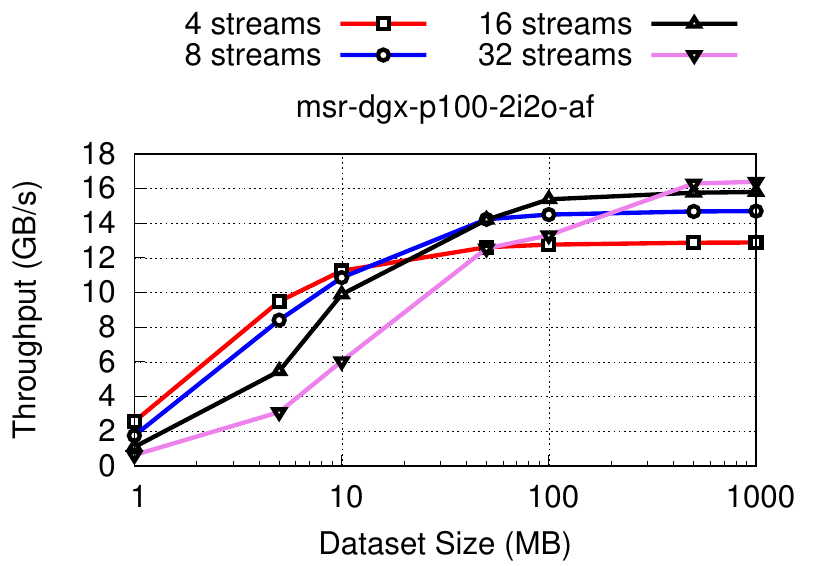}}
\subfigure[MCA]{\label{fig:msr-dgx-p100-mc-af} 
\includegraphics[width=0.32\textwidth]{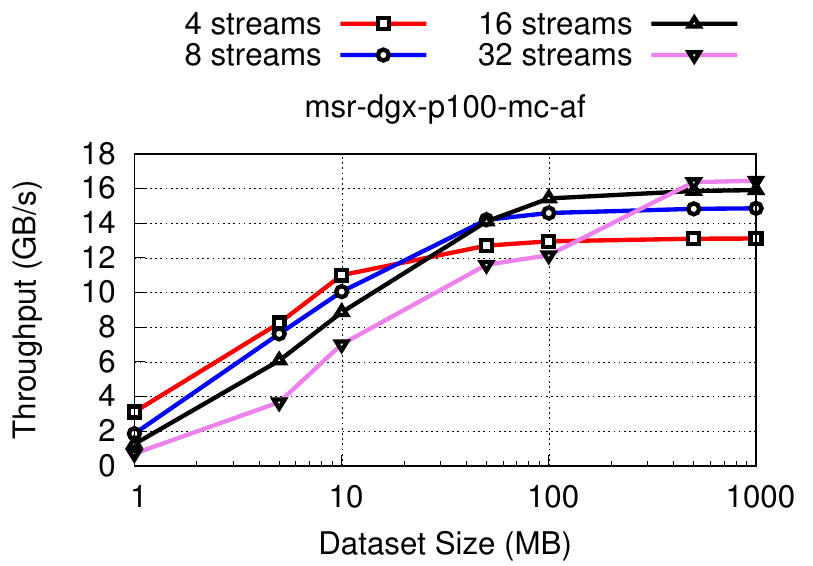}}
\vspace{-3mm}
\label{fig:msr-dgx-p100-mimo-mca}
\caption{msr-dgx-p100 MIMO MCA}
\vspace{-3mm}
\end{figure*}

\begin{figure*}[h]
\centering
\subfigure[3 GPU chain forward]{\label{fig:msr-dgx-p100-3-chain-f}
\includegraphics[width=0.32\textwidth]{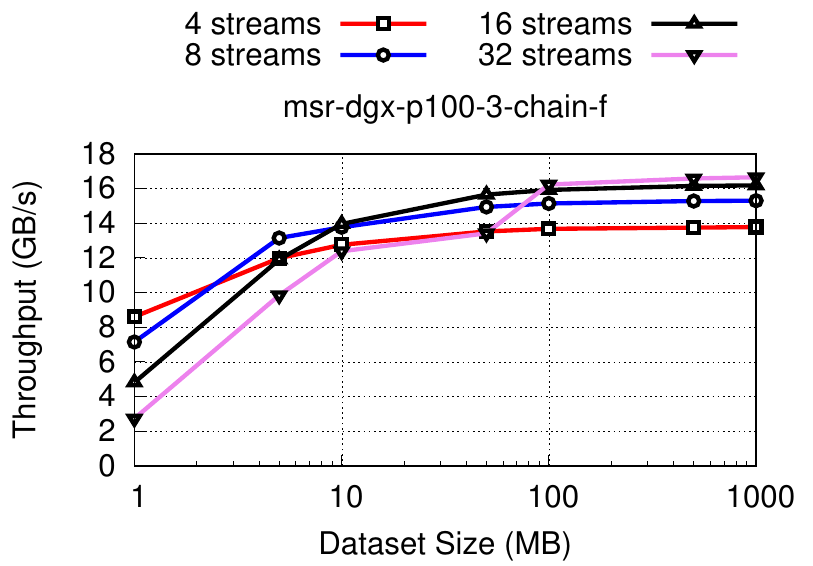}}
\subfigure[3 GPU chain reduce+forward]{\label{fig:msr-dgx-p100-3-chain-af} 
\includegraphics[width=0.32\textwidth]{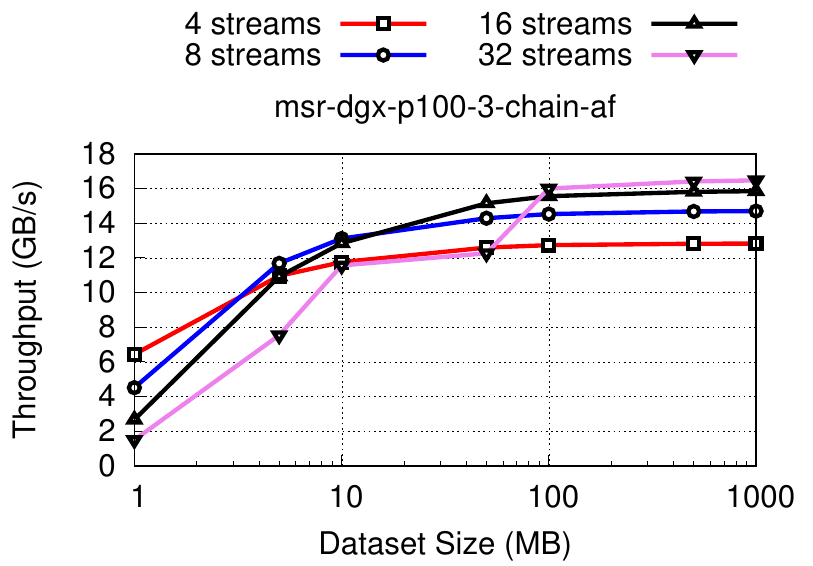}}
\subfigure[3 GPU chain reduce+bcast]{\label{fig:msr-dgx-p100-3-reduce-bcast} 
\includegraphics[width=0.32\textwidth]{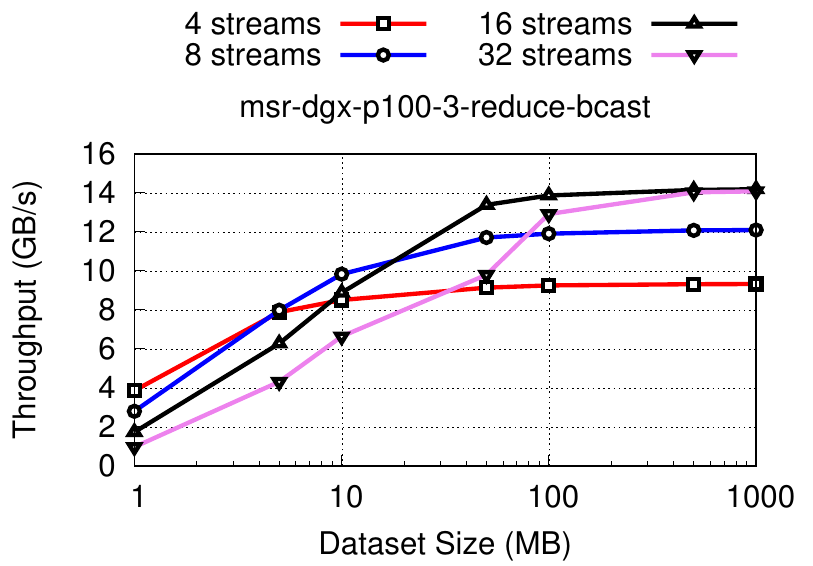}}
\subfigure[4 GPU chain forward]{\label{fig:msr-dgx-p100-4-chain-f}
\includegraphics[width=0.32\textwidth]{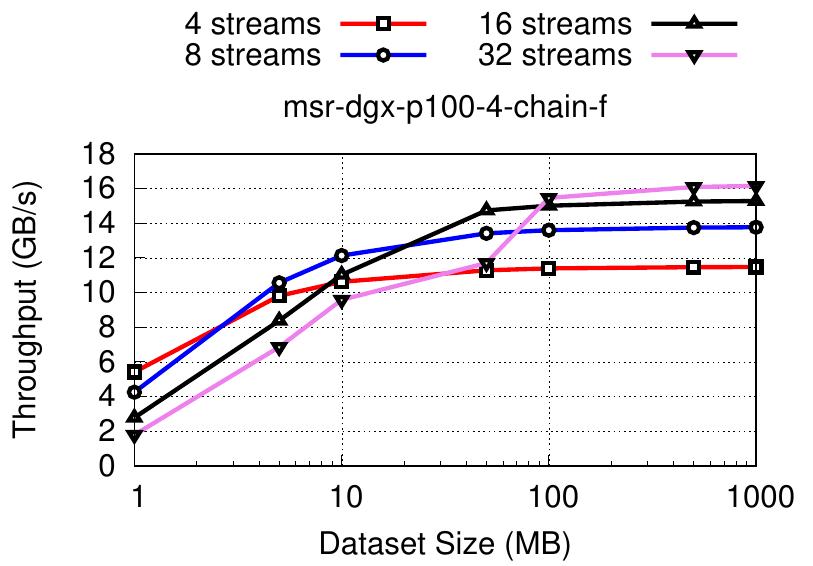}}
\subfigure[4 GPU chain reduce+forward]{\label{fig:msr-dgx-p100-4-chain-af} 
\includegraphics[width=0.32\textwidth]{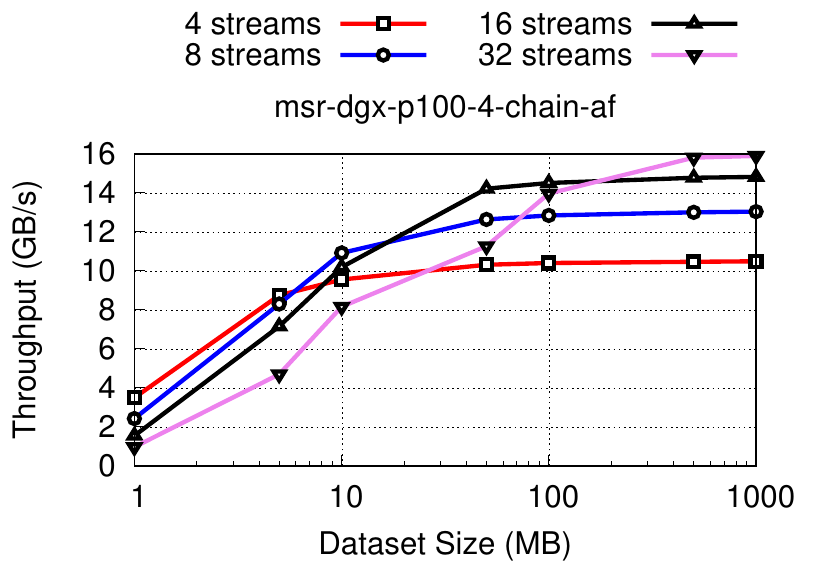}}
\subfigure[4 GPU chain reduce+bcast]{\label{fig:msr-dgx-p100-4-reduce-bcast} 
\includegraphics[width=0.32\textwidth]{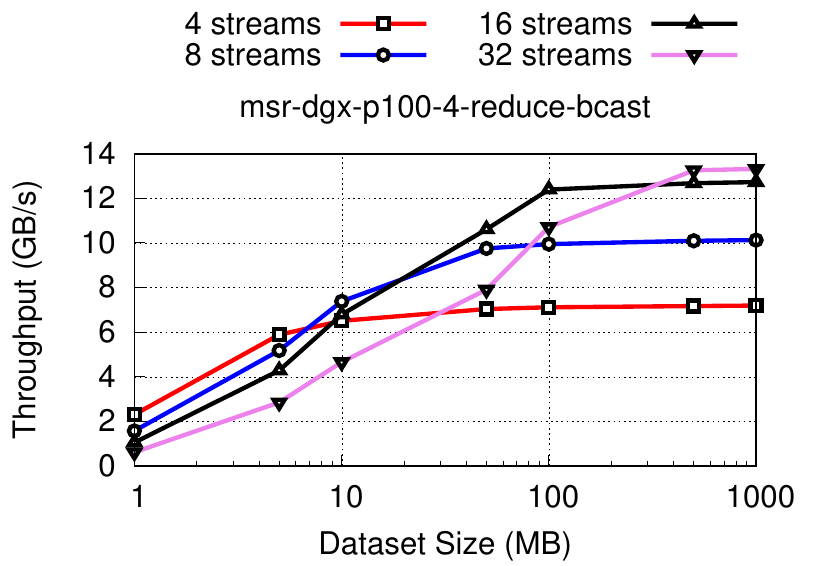}}
\subfigure[5 GPU chain forward]{\label{fig:msr-dgx-p100-5-chain-f}
\includegraphics[width=0.32\textwidth]{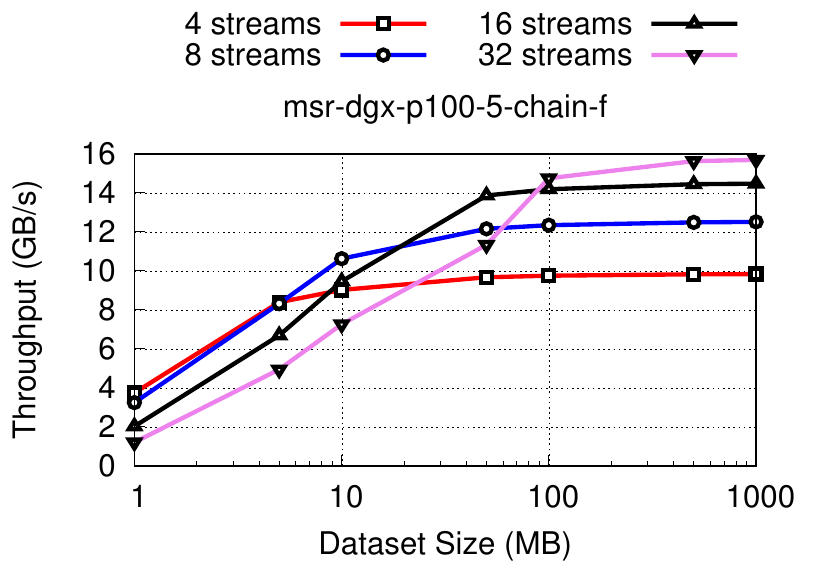}}
\subfigure[5 GPU chain reduce+forward]{\label{fig:msr-dgx-p100-5-chain-af} 
\includegraphics[width=0.32\textwidth]{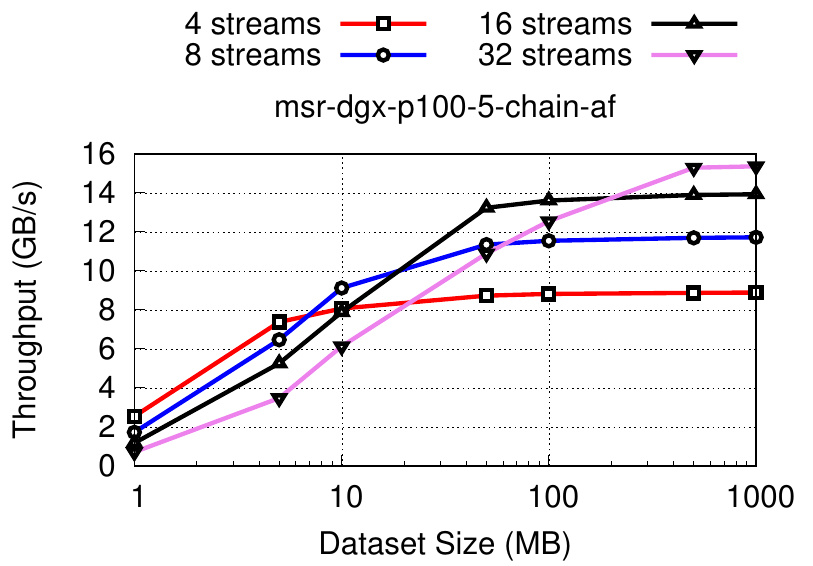}}
\subfigure[5 GPU chain reduce+bcast]{\label{fig:msr-dgx-p100-5-reduce-bcast} 
\includegraphics[width=0.32\textwidth]{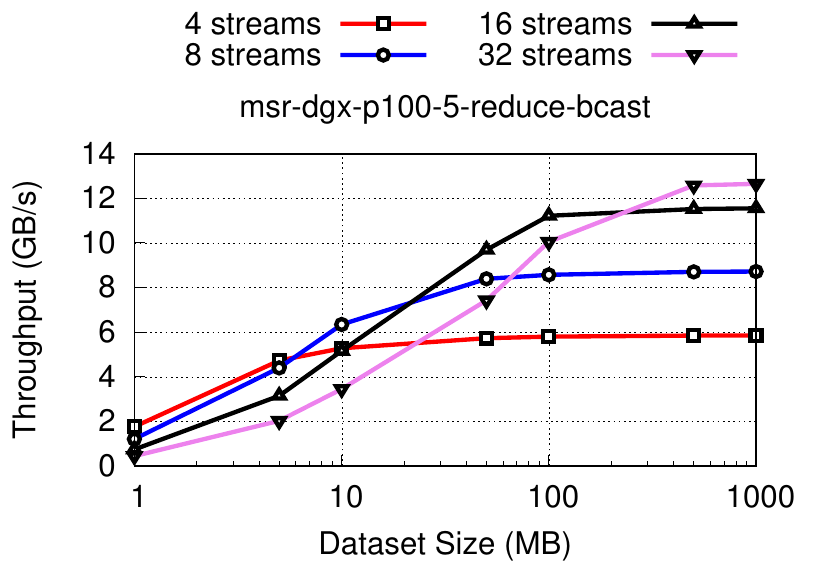}}
\vspace{-3mm}
\label{fig:msr-dgx-p100-345-chain}
\caption{msr-dgx-p100 3,4,5 chain forward, reduce+forward, reduce-bcast}
\vspace{-3mm}
\end{figure*}

\begin{figure*}[h]
\centering
\subfigure[6 GPU chain forward]{\label{fig:msr-dgx-p100-6-chain-f}
\includegraphics[width=0.32\textwidth]{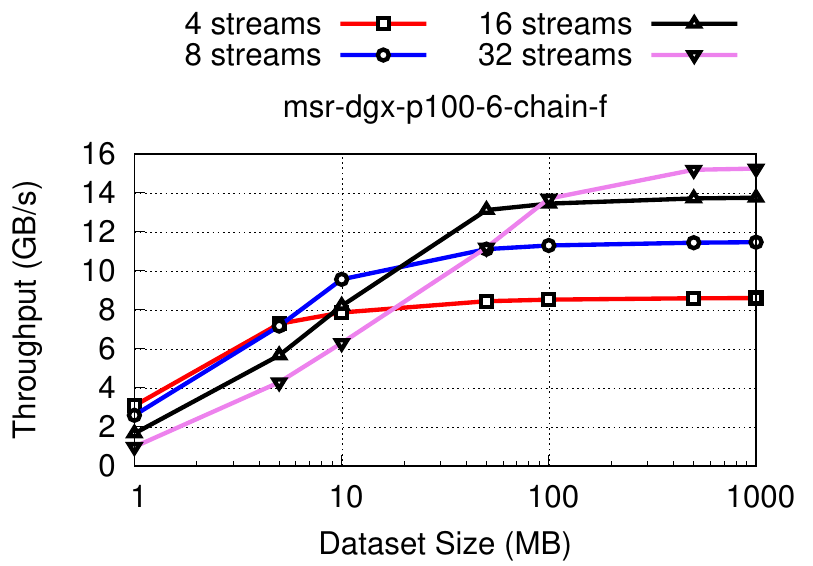}}
\subfigure[6 GPU chain reduce+forward]{\label{fig:msr-dgx-p100-6-chain-af} 
\includegraphics[width=0.32\textwidth]{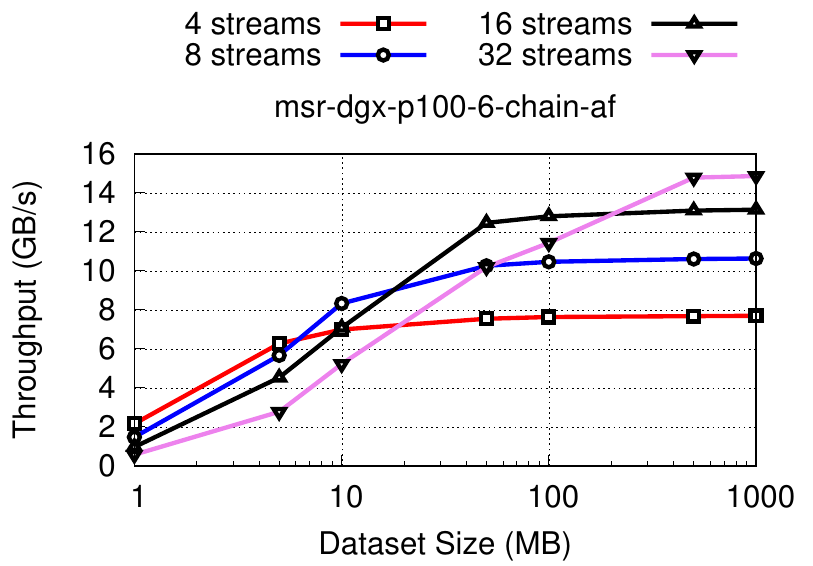}}
\subfigure[6 GPU chain reduce+bcast]{\label{fig:msr-dgx-p100-6-reduce-bcast} 
\includegraphics[width=0.32\textwidth]{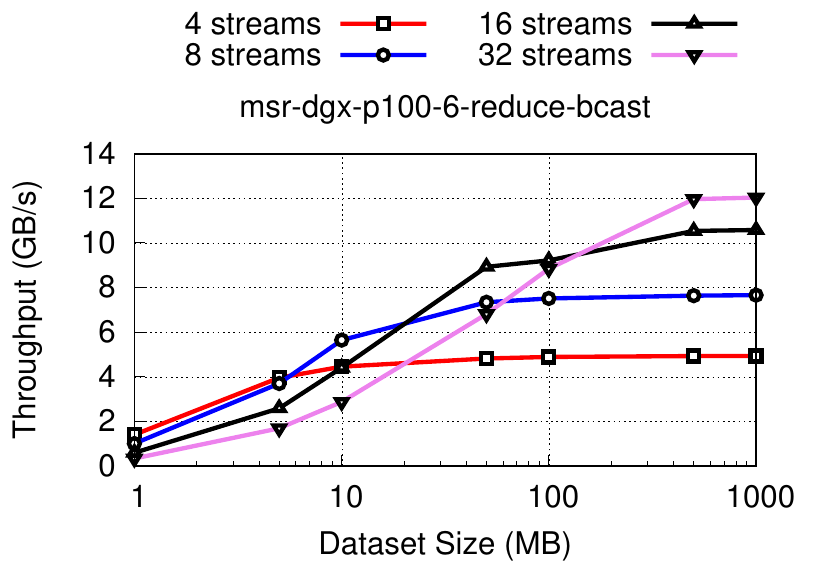}}

\subfigure[7 GPU chain forward]{\label{fig:msr-dgx-p100-7-chain-f}
\includegraphics[width=0.32\textwidth]{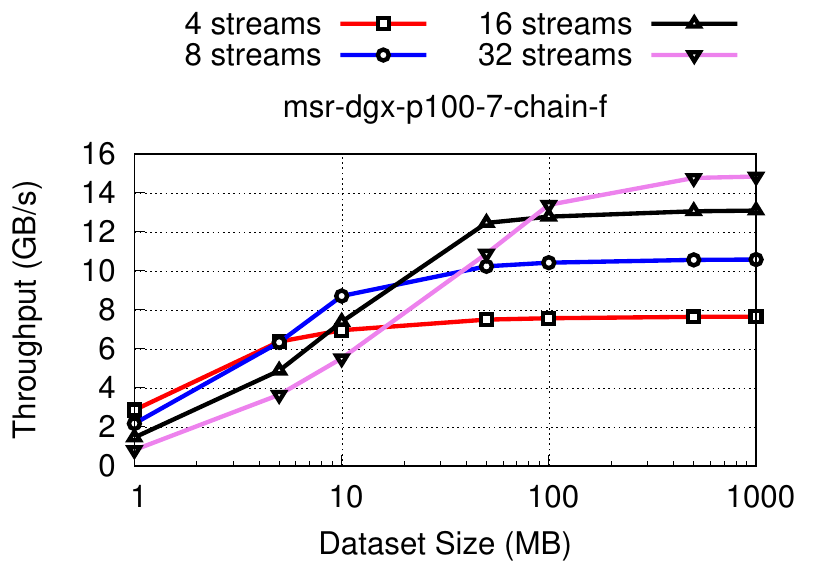}}
\subfigure[7 GPU chain reduce+forward]{\label{fig:msr-dgx-p100-7-chain-af} 
\includegraphics[width=0.32\textwidth]{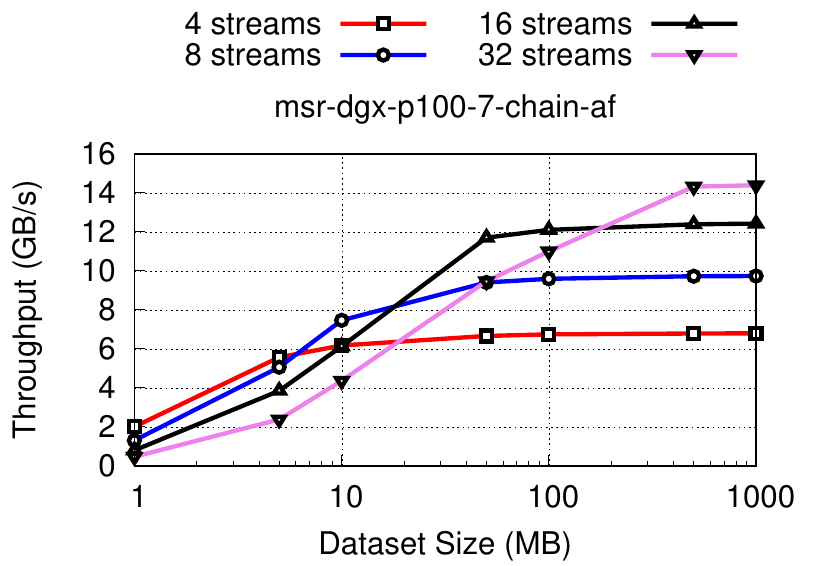}}
\subfigure[7 GPU chain reduce+bcast]{\label{fig:msr-dgx-p100-7-reduce-bcast} 
\includegraphics[width=0.32\textwidth]{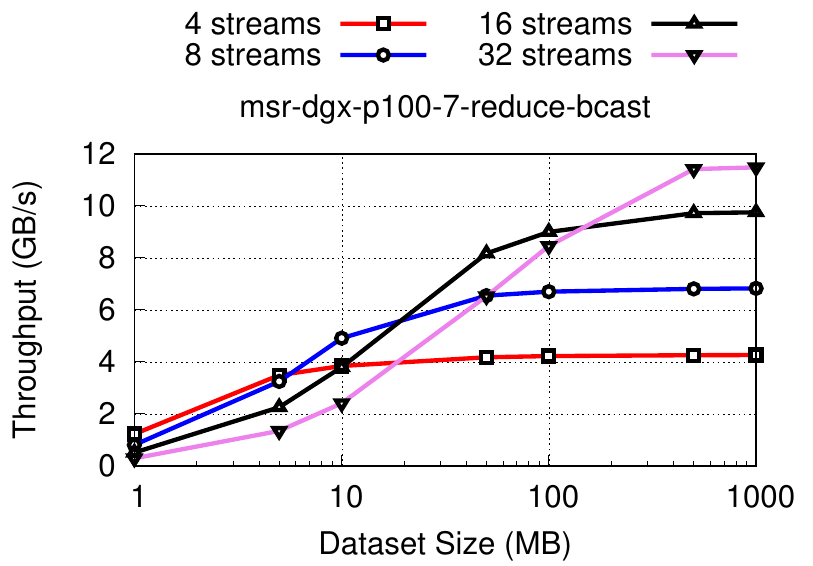}}

\subfigure[8 GPU chain forward]{\label{fig:msr-dgx-p100-8-chain-f}
\includegraphics[width=0.32\textwidth]{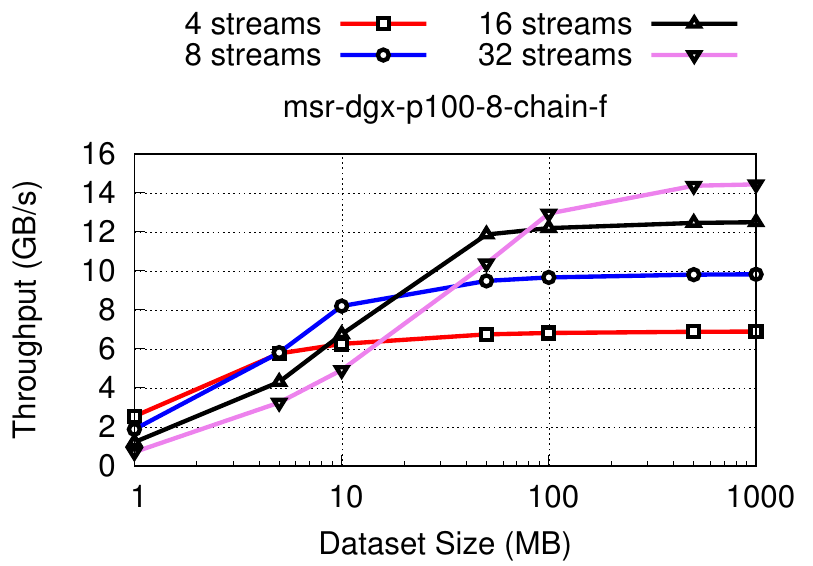}}
\subfigure[8 GPU chain reduce+forward]{\label{fig:msr-dgx-p100-8-chain-af} 
\includegraphics[width=0.32\textwidth]{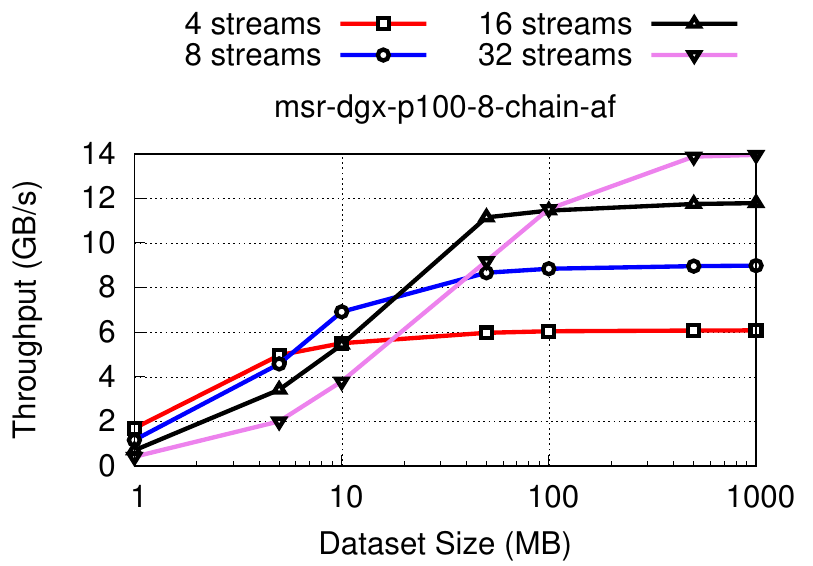}}
\subfigure[8 GPU chain reduce+bcast]{\label{fig:msr-dgx-p100-8-reduce-bcast} 
\includegraphics[width=0.32\textwidth]{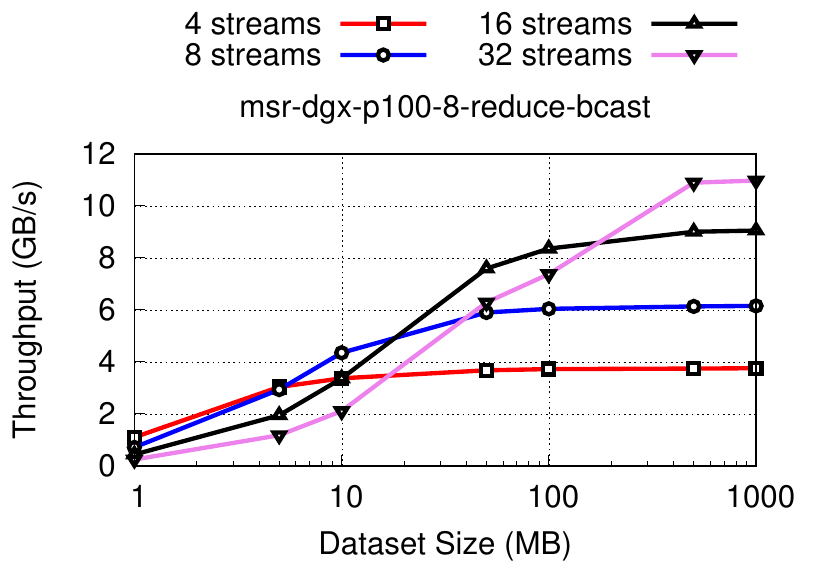}}
\vspace{-3mm}
\label{fig:msr-dgx-p100-678-chain}
\caption{msr-dgx-p100 6,7,8 chain forward, reduce+forward, reduce-bcast}
\vspace{-3mm}
\end{figure*}

%\begin{figure*}[h]
%\centering
%\subfigure[Broadcast]{\label{fig:msr-bcast}
%\includegraphics[width=0.5\columnwidth]{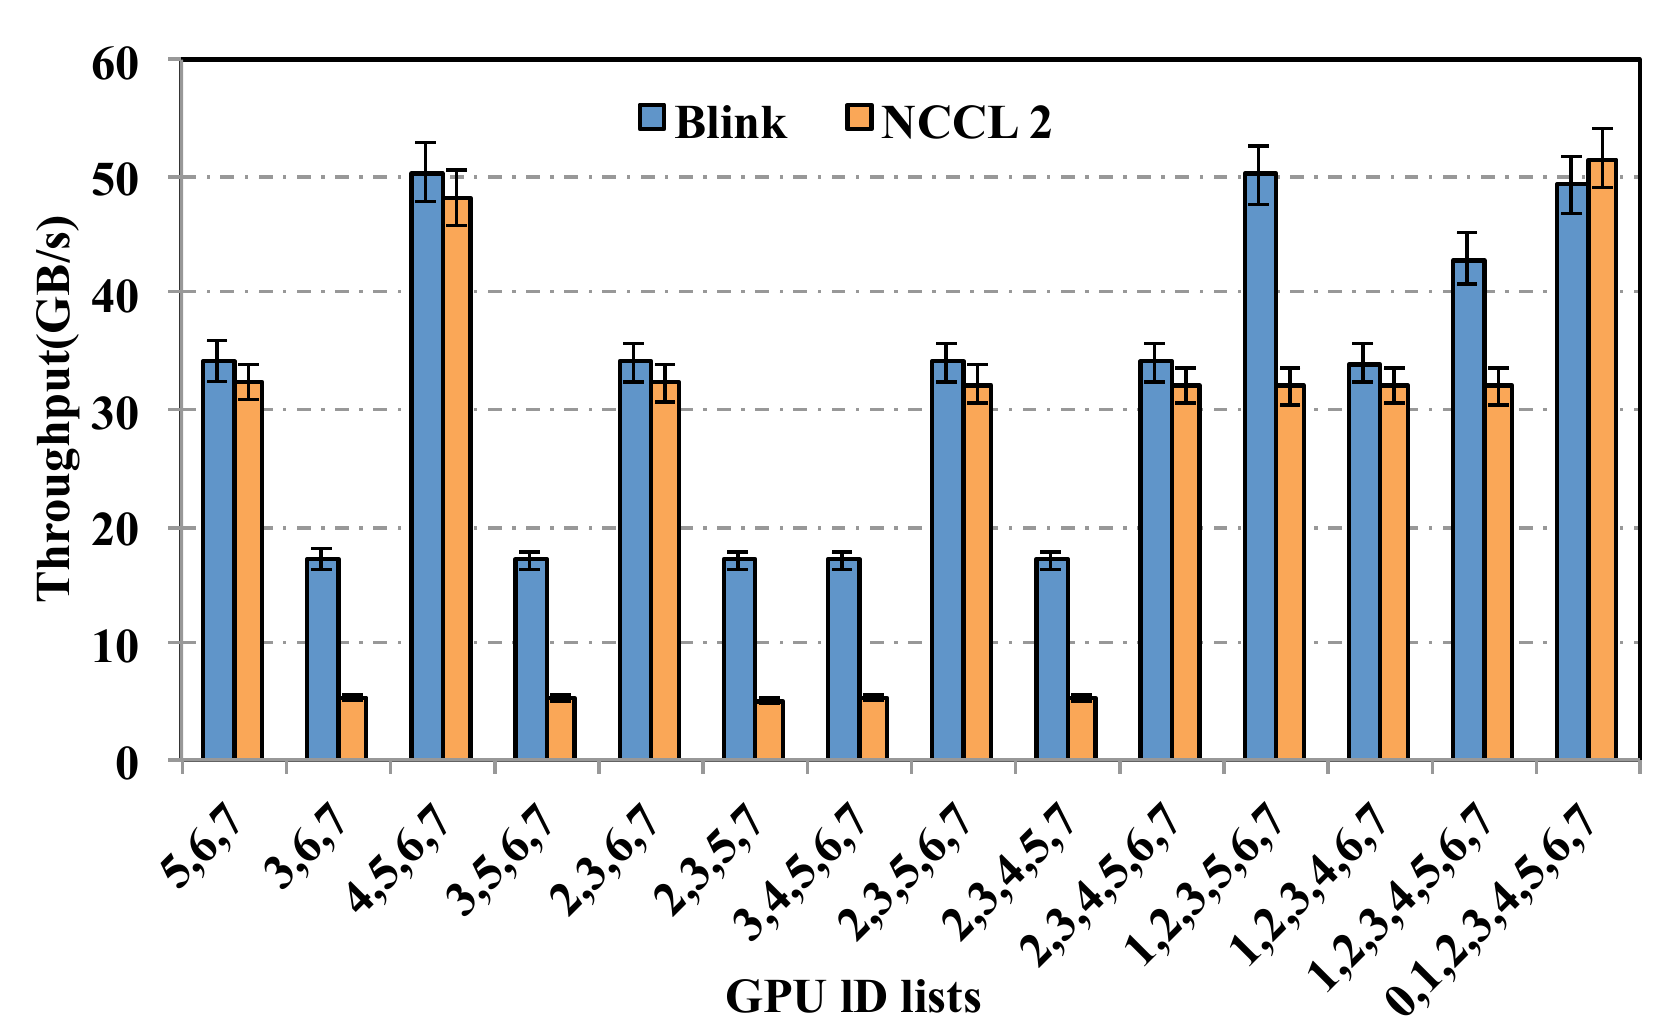}}
%\vspace{-3mm}
%\label{fig:msr-bcast}
%\caption{Broadcast comparison between NCCL2 and Blink in all possible topologies on Azure DGX-1 (P100)}
%\vspace{-3mm}
%\end{figure*}
\clearpage
\newpage
\subsection{Cross-machine (\dgxv)}

\begin{figure*}[!t]
\centering
\subfigure[40Gbps]{\label{fig:40Gbps}
\includegraphics[width=0.32\textwidth]{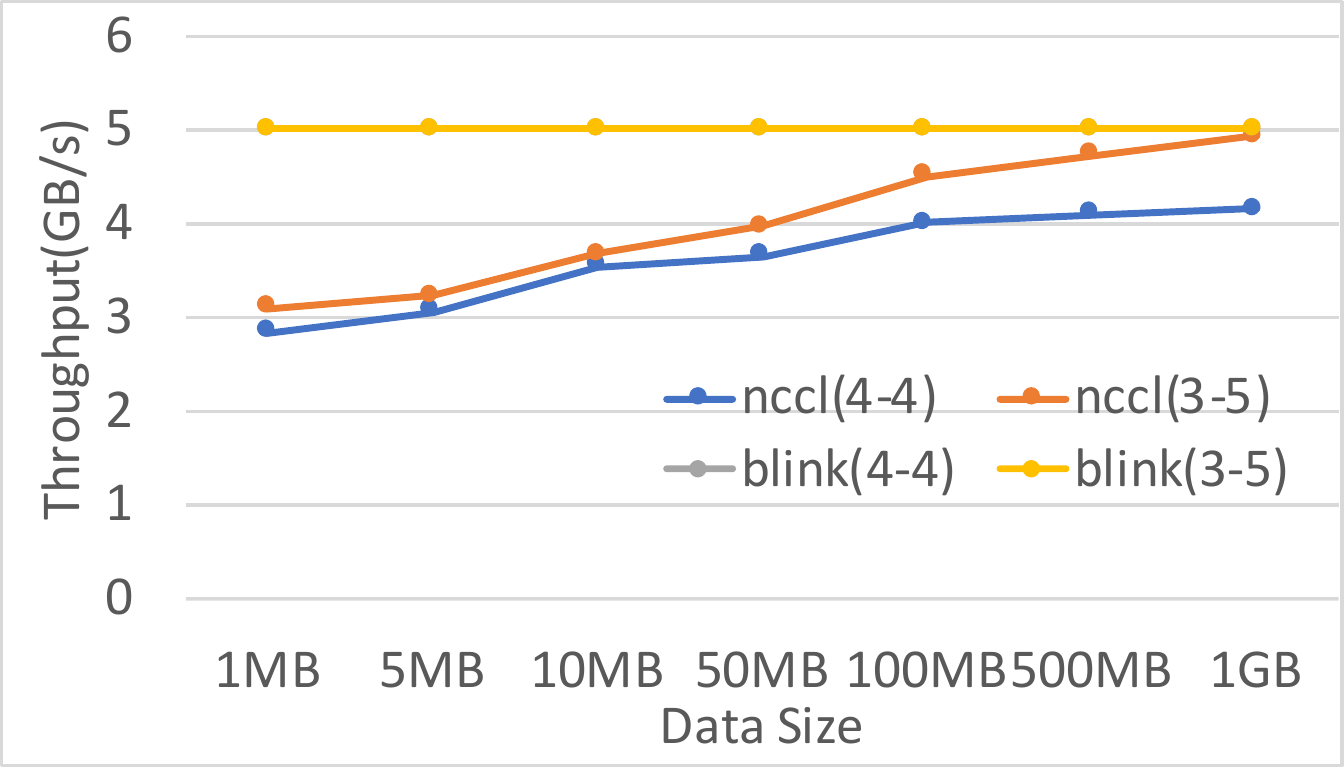}}
\subfigure[100Gbps]{\label{fig:100Gbps} 
\includegraphics[width=0.32\textwidth]{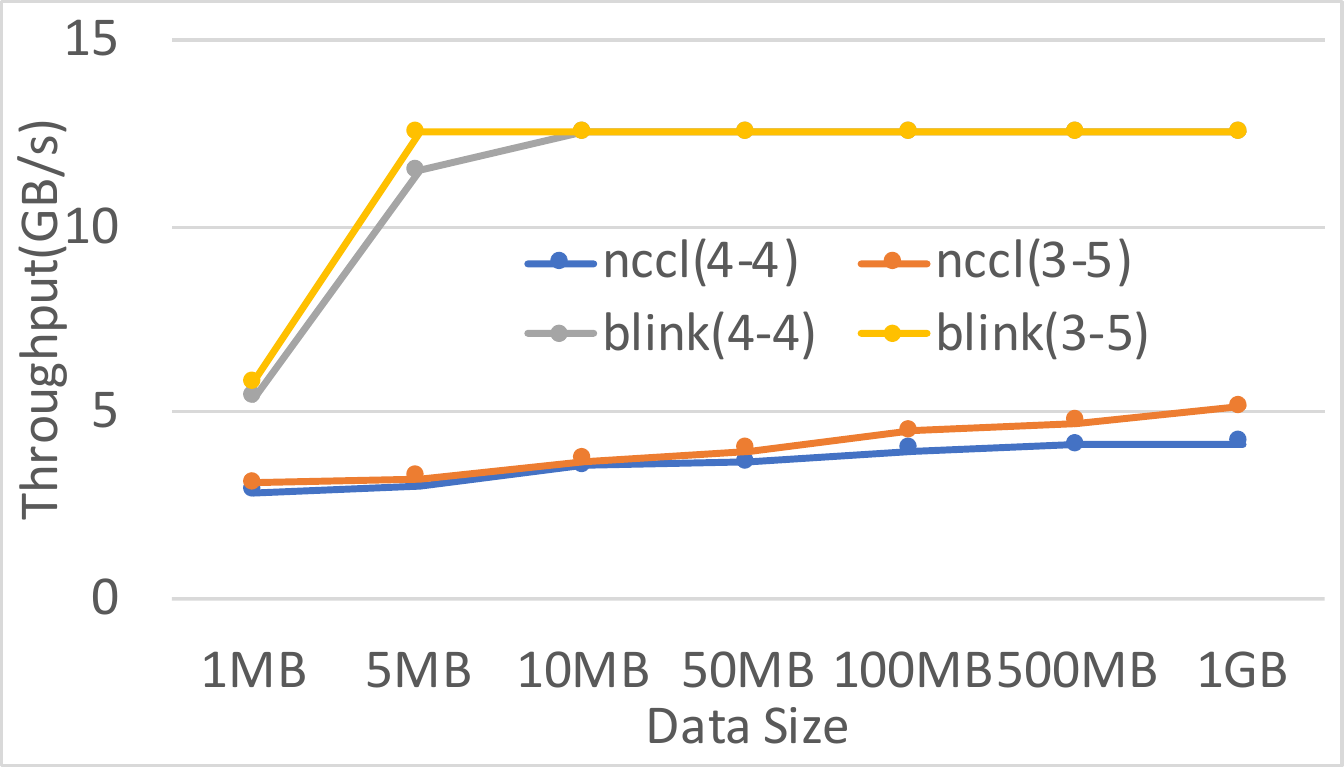}}
\subfigure[400Gbps]{\label{fig:400Gbps} 
\includegraphics[width=0.32\textwidth]{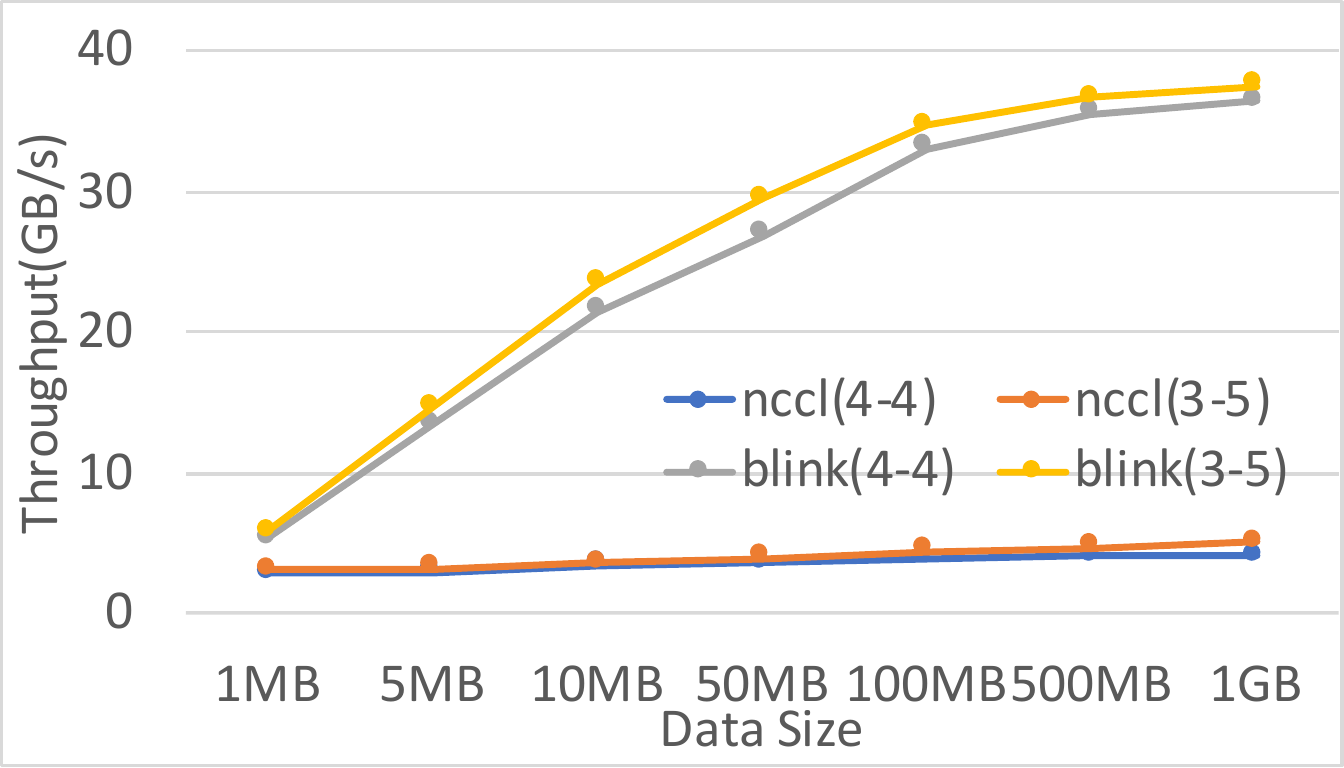}}

\subfigure[10MB]{\label{fig:10MB-crossmachine}
\includegraphics[width=0.32\textwidth]{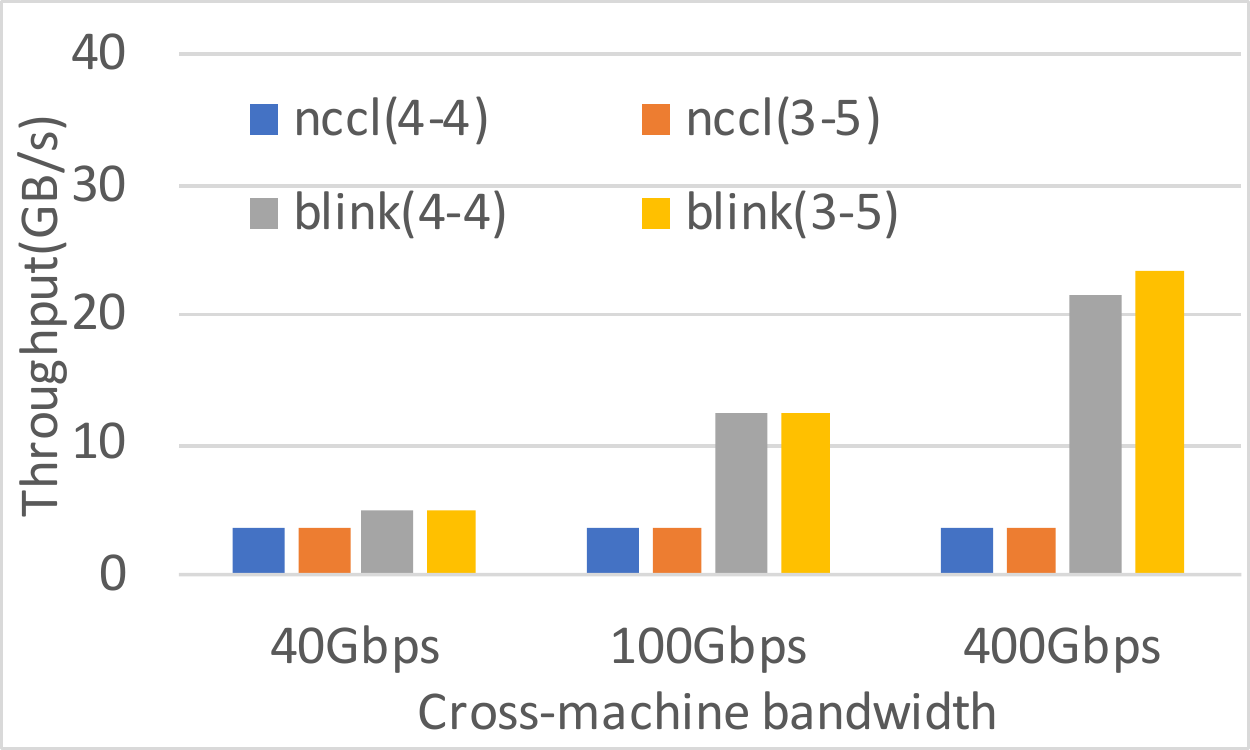}}
\subfigure[100MB]{\label{fig:100MB-crossmachine}
\includegraphics[width=0.32\textwidth]{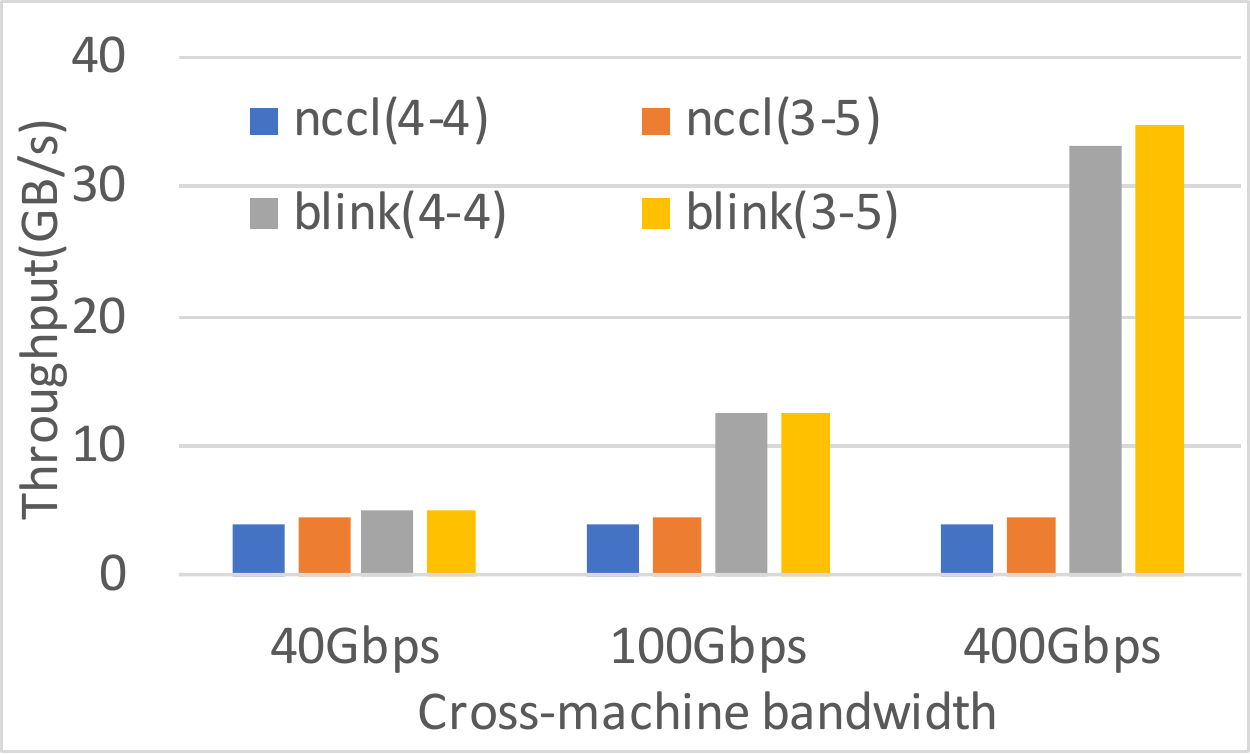}}
\subfigure[1GB]{\label{fig:1GB-crossmachine} 
\includegraphics[width=0.32\textwidth]{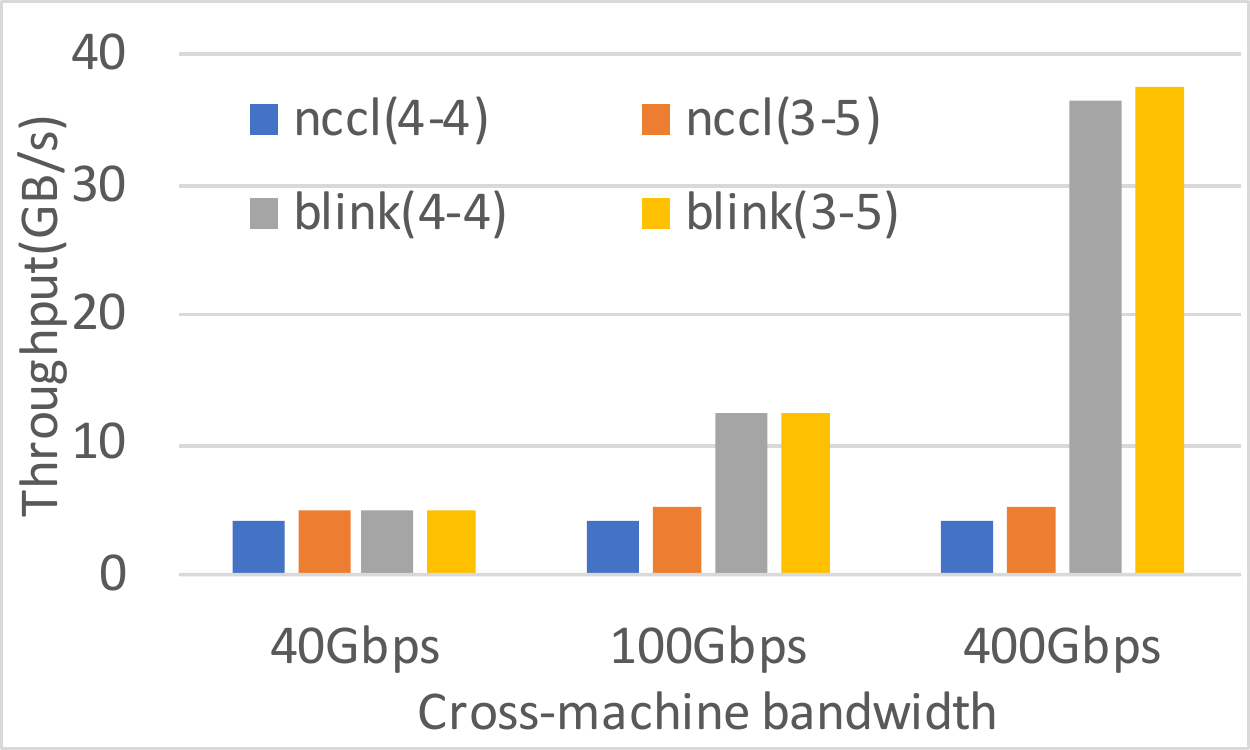}}
\label{fig:cross-machine-simulation}
\caption{Cross-machine (2 DGX-1) simulation with varied inter-machine link bandwidth.}
\end{figure*}

\begin{figure}[t!]
\centering
\includegraphics[width=0.99\columnwidth]{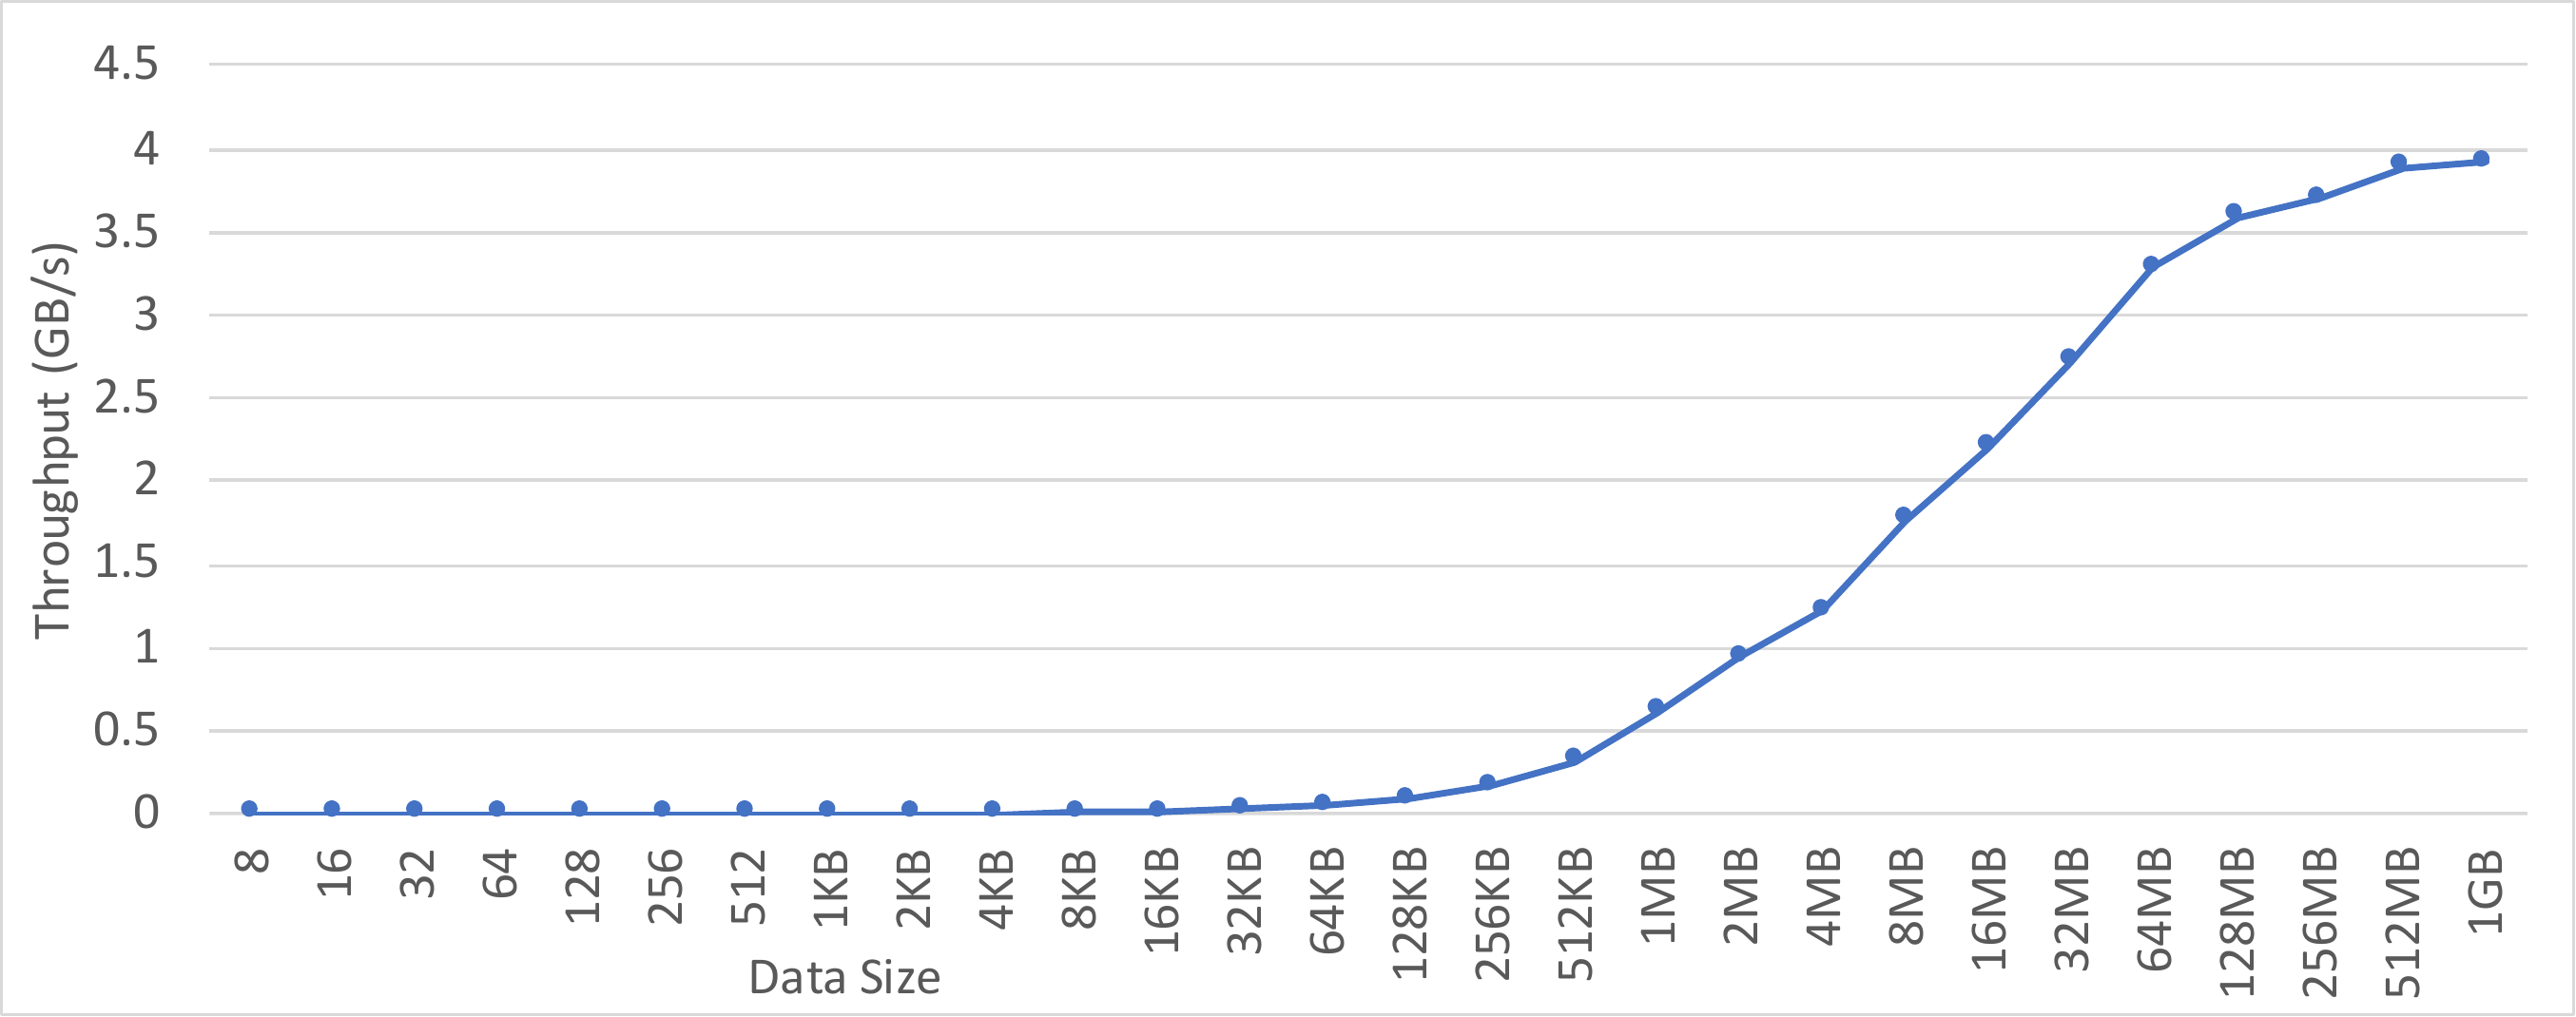}
\label{fig:nccl-2-dgx1}
\caption{Throughput across 2 \dgxv machines using NCCL}
\end{figure}

% \begin{figure}[h]
% \centering
% \includegraphics[width=0.99\columnwidth]{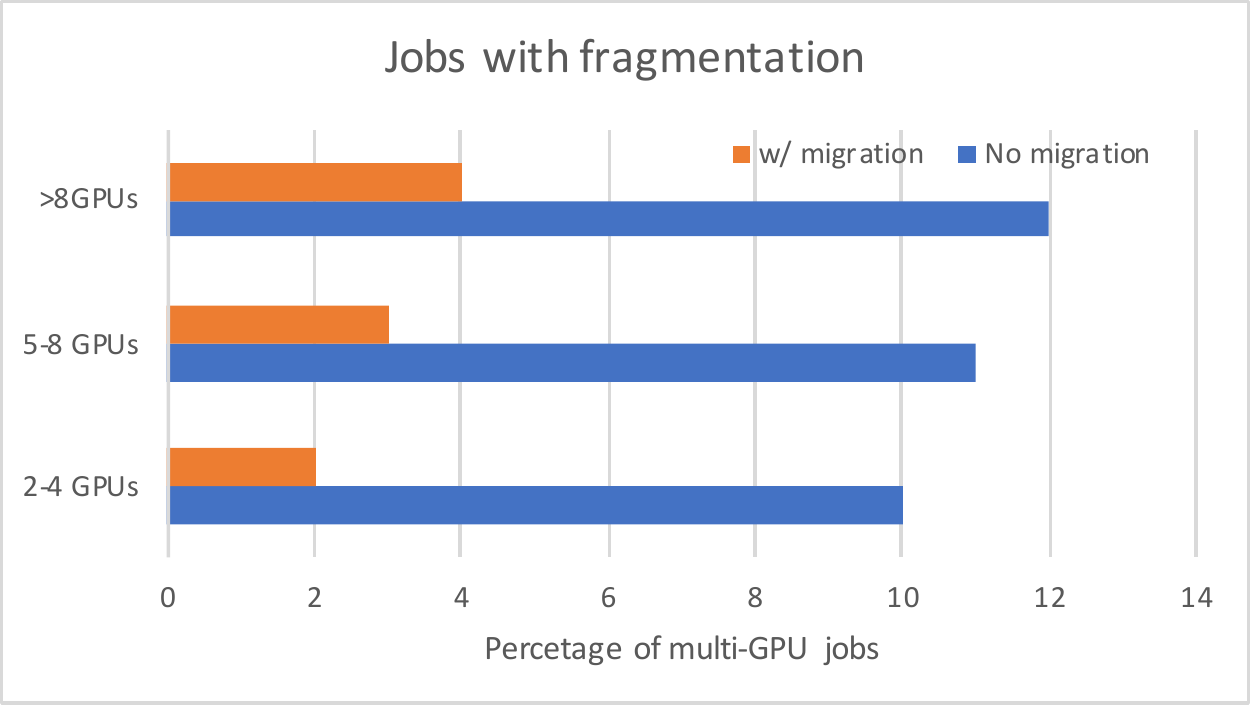}
% \label{fig:pack-frag}
% \caption{[Placeholder (fake) graph] Effect of job migration and packing on fragmentation (Philly traces).}
% \end{figure}
